# Supplementary material for: Motion-X++: A Large-Scale Multimodal 3D Whole-body Human Motion Dataset
Source: arXiv:2501.05098 source file (2025-01-09)
Supplement: Supplementary file 1 [file 6_supp.tex]

%\appendix
\section*{Appendix}

\section{Motion-X: Additional Details}
In this section, we provide more details about \newdataname that are not included in the main paper due to space limitations, including statistic analyses, data preprocessing, and motion augmentation mechanism.

\subsection{Statistic Analyses}

Fig.~\ref{fig:data_comp_sup} (a) shows each sub-dataset standard deviation of body, hand, and face joints. Our dataset has a large diversity of the hand and face joints, filling the gap of the previous body-only dataset in terms of expressiveness. Besides, as shown in Fig.~\ref{fig:data_comp_sup} (b), \dataname provides a large volume of long motion ($>240$ frames), which will be beneficial for long-term motion generation.

\begin{figure*}[h]	
    \centering
    %\vspace{-0.2cm}
        %\subfigure[Motion diversity] 
        % {
        %     \begin{minipage}[t]{0.5\linewidth}
        %         %\centering      
        %         \includegraphics[width=3.4in]{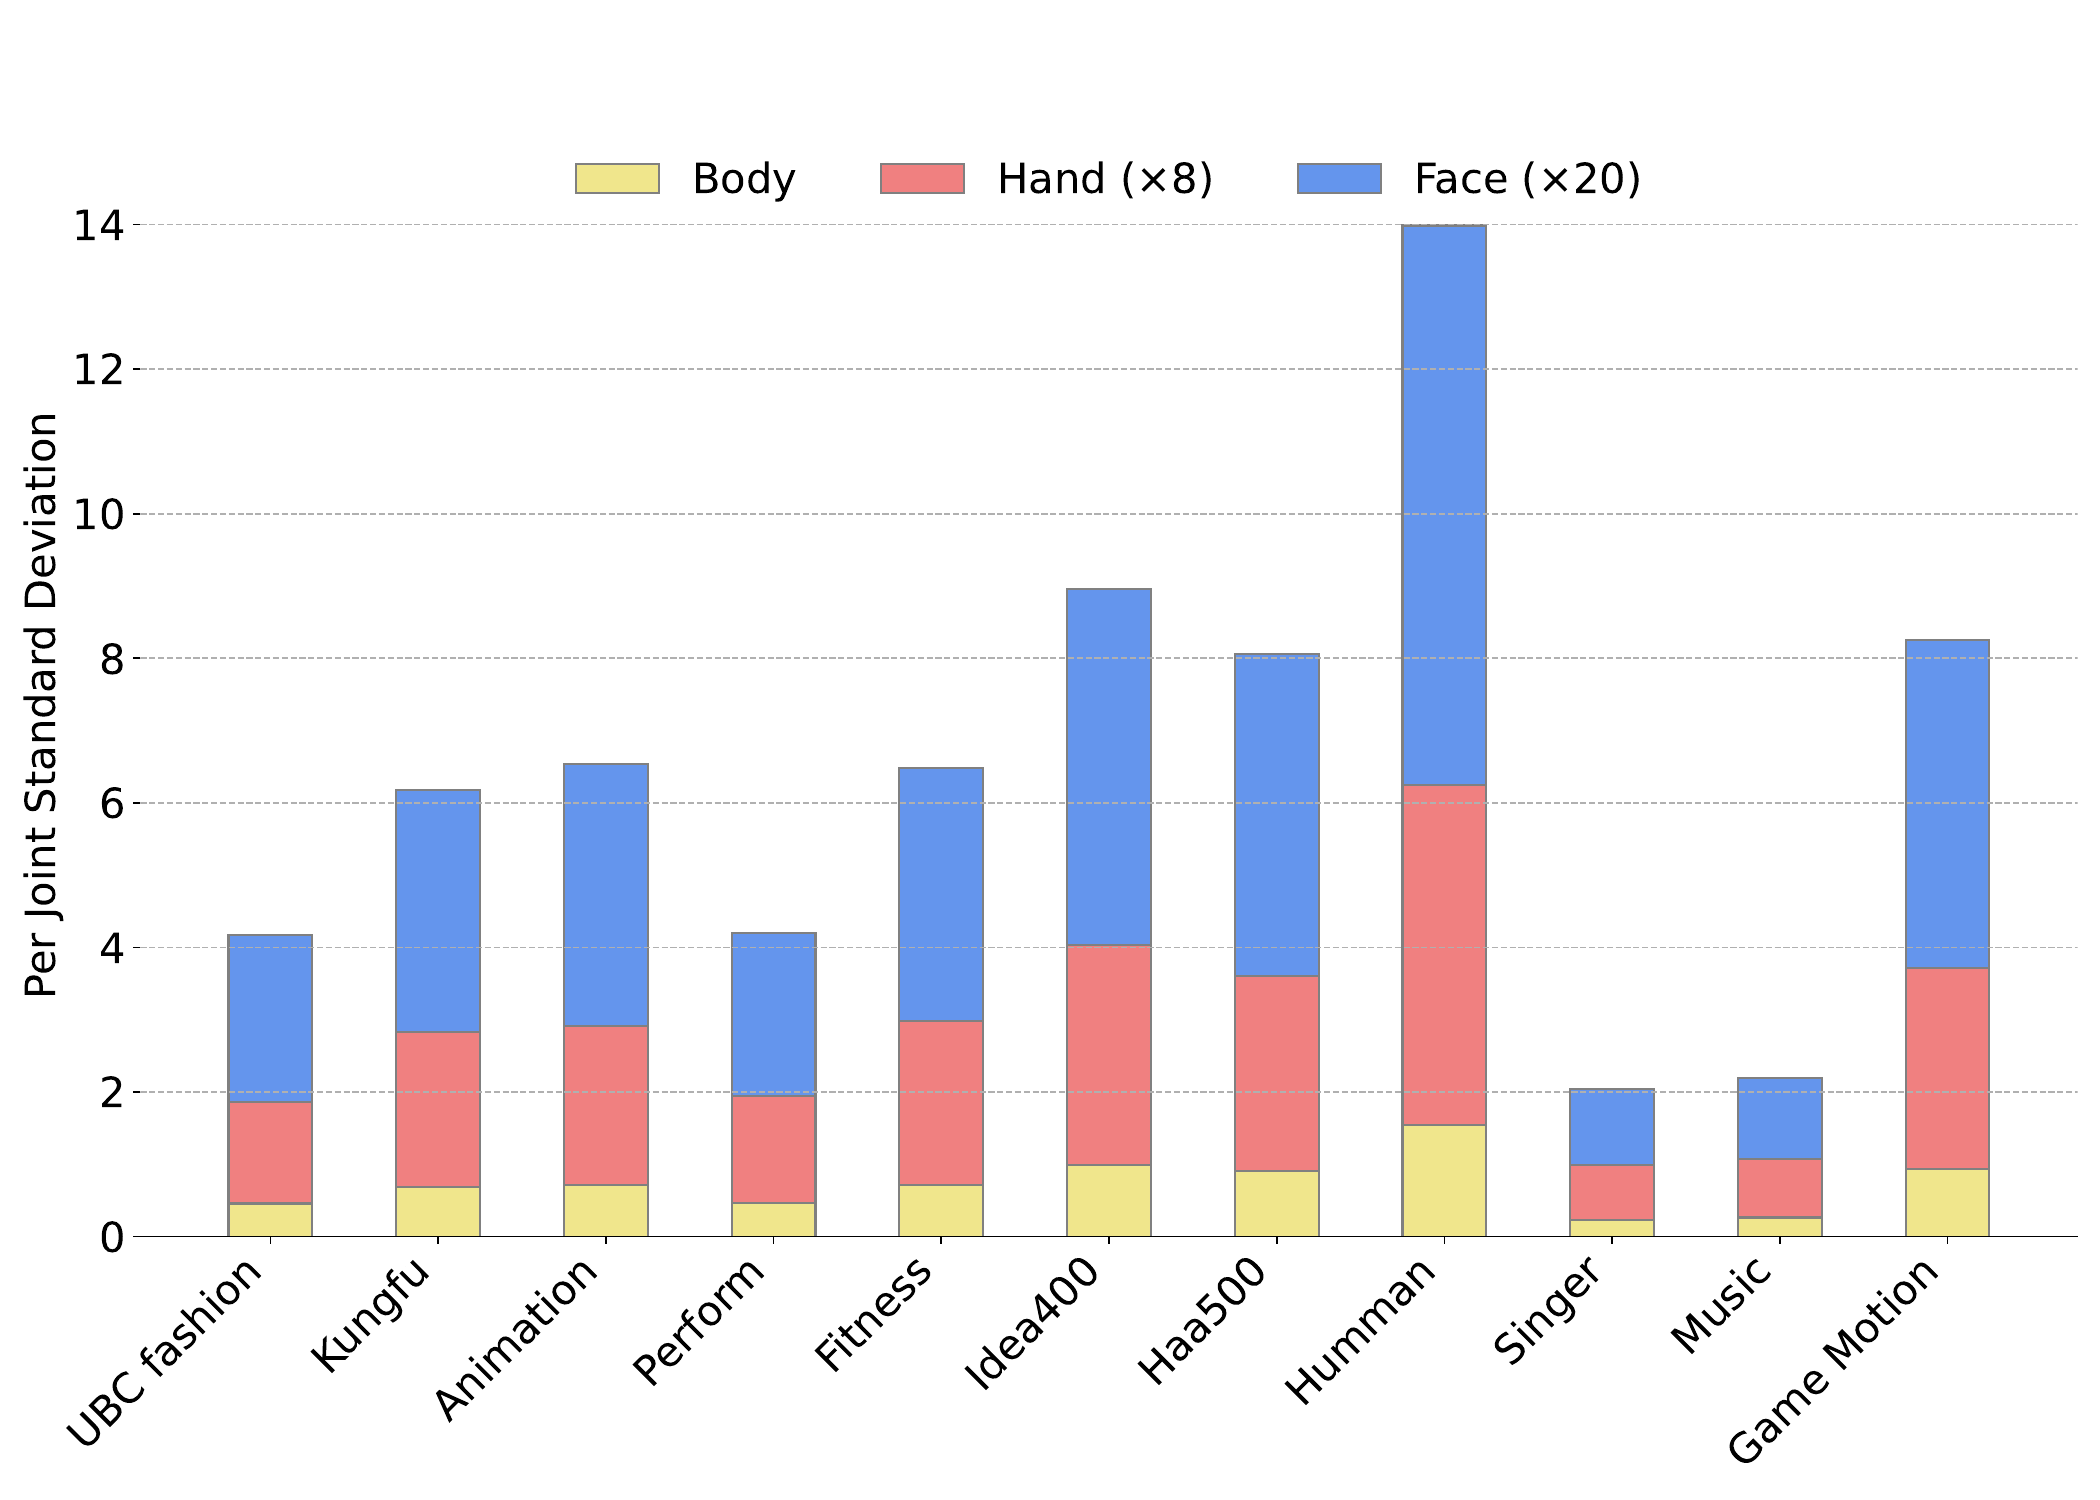}
        %     \end{minipage}
        % }
        %     \label{fig:std_data}  
        %     \hspace{1cm}
        % {
        %     \begin{minipage}[t]{0.3\linewidth}
        %         \centering         
        %         \includegraphics[width=2.5in]{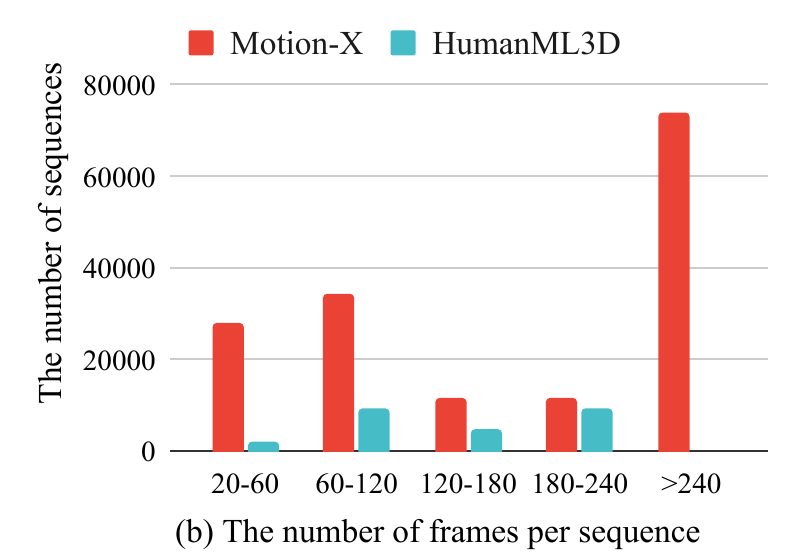}   
        %     \end{minipage}
        % } 
        \begin{center}
        \includegraphics[width=1\textwidth]{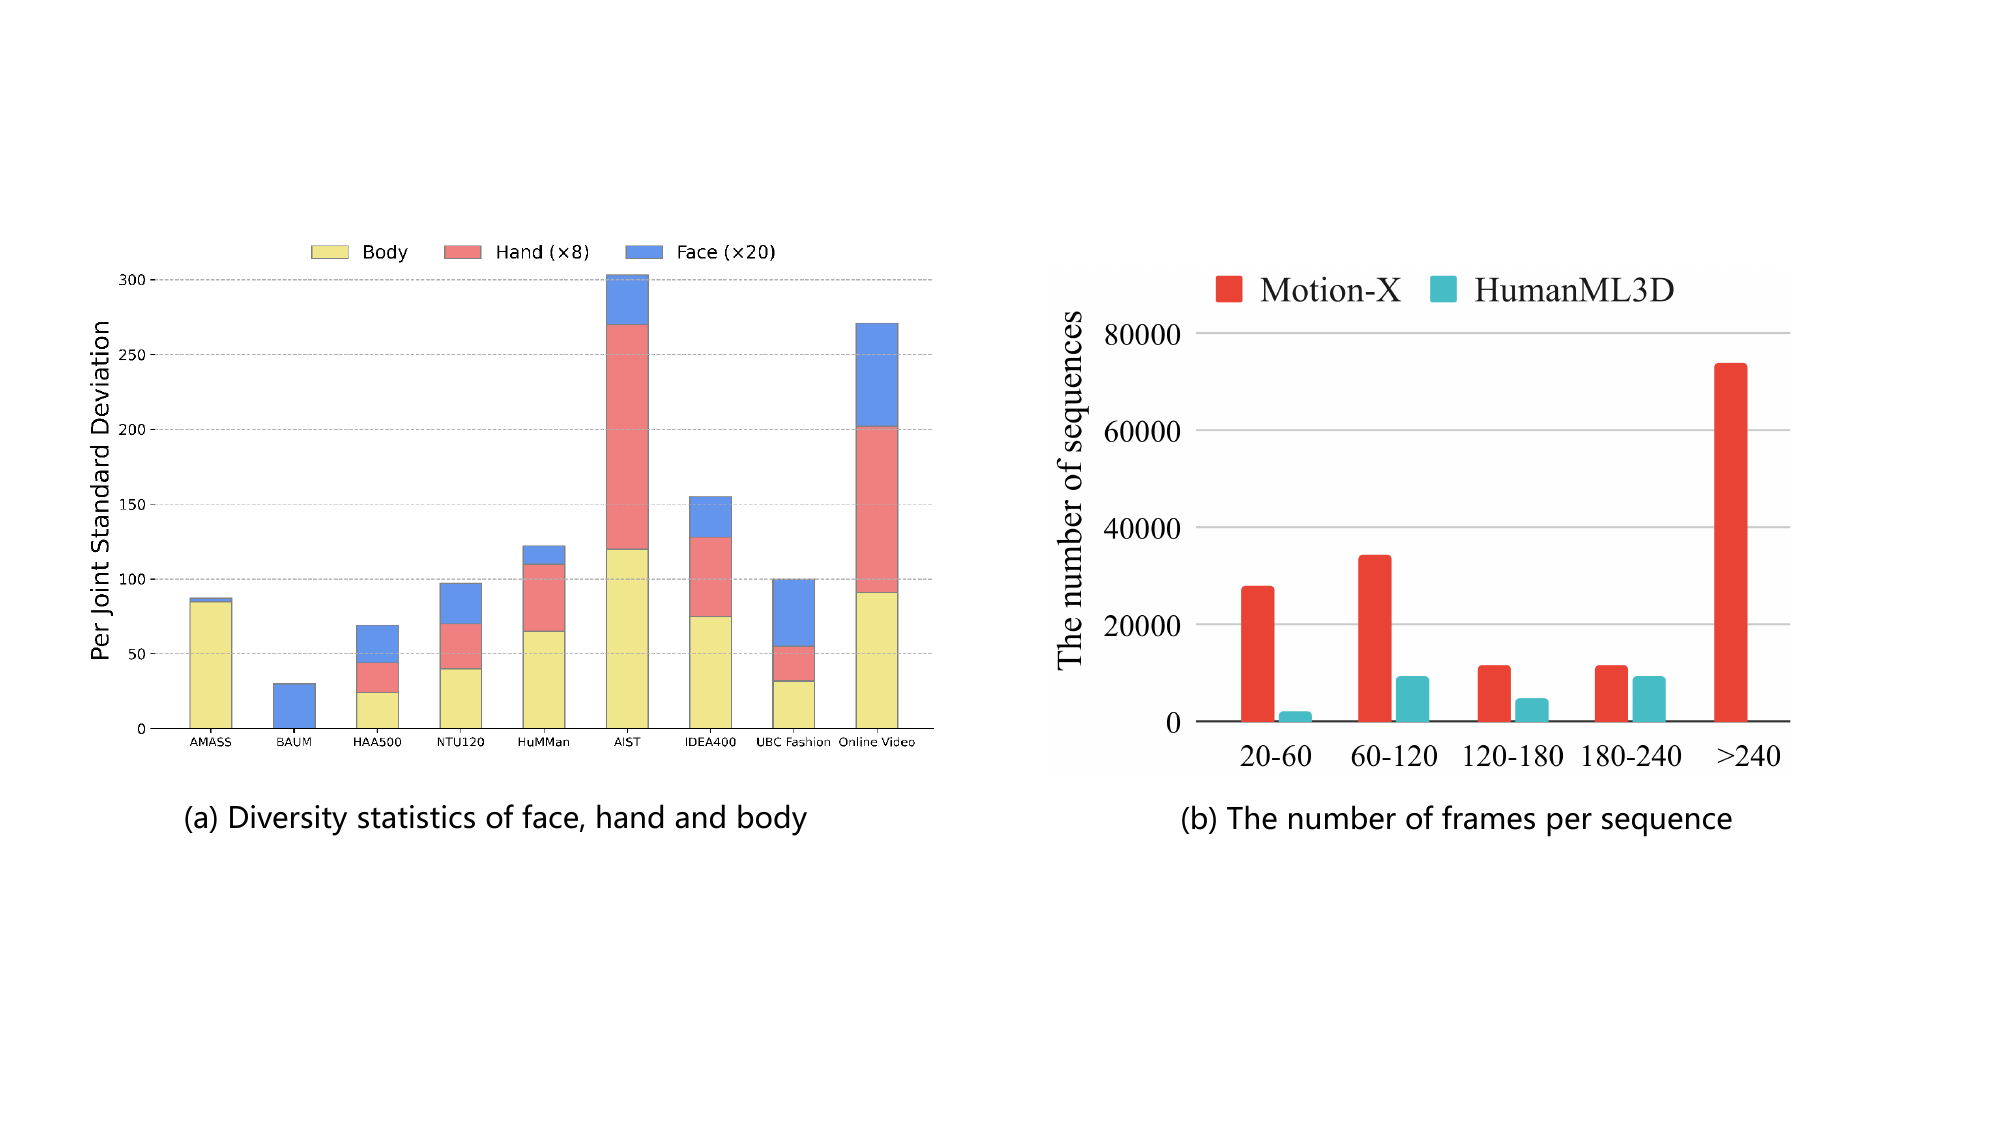}
    \end{center}
            \label{fig:frame_data} 
    \vspace{0.2cm}
    \caption{Statistics of motion diversity and length.}
    \vspace{-0.4cm}
    \label{fig:data_comp_sup} 
    \end{figure*}

\subsection{Processing of Each Sub-dataset}

We gather 81.1K motion sequences from seven existing datasets and a large volume of online videos with the proposed annotation pipeline. As shown in Tab.~\ref{tab:statistic_subdataset}, due to the lack of comprehensive annotations from their original datasets, we provide well-annotated whole-body motion, comprehensive semantic labels, and whole-body pose descriptions for all datasets. Here we introduce more details about each sub-dataset's data preprocessing.

\begin{table*}[h]
	\vspace{4pt}
        \centering
	\resizebox{0.9\textwidth}{!}{%
    \begin{tabular}{lccccc}
        \toprule
            \rowcolor{color3} \text{Dataset} &~~~\text{Clip Number}~~~ & ~~\text{Frame Number}~~ & \text{Motion Annotation} & \text{Text Annotation} & \text{RGB} \\        \midrule
            AMASS~\cite{humanml3d} & 26.3K & 5.4M & B,H & S & \xmark \\ 
            AIST~\cite{tsuchida2019aist} & 1.4K & 0.3M & B & S &  \cmark\\
            HAA500~\cite{chung2021haa500} & 5.2K & 0.3M & - & S &  \cmark \\ 
            HuMMan~\cite{cai2022humman} & 0.7K & 0.1M & B & S &  \cmark \\
            GRAB~\cite{taheri2020grab} & 1.3K & 0.4M & B,H & S  & \xmark\\ 
            EgoBody~\cite{zhang2022egobody} & 1.0K & 0.4M & B,H & - &  \cmark \\ 
            BAUM~\cite{baum} & 1.4K & 0.2M & F & S  & \cmark\\ 
            UBC Fashion~\cite{UBCdwnet} & 0.5K & 0.2M & - & - & - \\
            IDEA400* & 12.5K & 2.6M & - & - &  \cmark \\
            Online Videos* & 68.3K & 9.4M & - & - &  \cmark\\ \midrule
            Motion-X++ & 120.5K & 19.5M & B,H,F & S,P & \cmark \\ \bottomrule
        \end{tabular}
	}
	\caption{\small Statistics of sub-datasets. B, H, and F are body, hand, and face. S and P are semantic and pose texts. Please note that the semantic text annotations are different from different datasets. Some action datasets~\cite{liu2019ntu,amass,chung2021haa500,baum} only provide action-level texts instead of sentences. Most semantic labels are annotated manually, making specific domain descriptions (e.g., specific instruments) hard to label precisely.  * denotes videos are collected in this work.}
	\label{tab:statistic_subdataset}
\vspace{-0.3cm}
\end{table*}
\textbf{AMASS}~\cite{amass} is the existing largest-scale motion capture dataset, which provides body motions and almost static hand motions. To fill in the face parameters, we extract facial expressions from the facial dataset BAUM~\cite{baum} with the SOTA facial reconstruction method EMOCA~\cite{emoca} and perform a data augmentation (in Sec.~\ref{sec:motion_aug}). For the text labels, we utilize the semantic labels from HumanML3D~\cite{humanml3d} and annotate the pose description with our whole-body pose captioning module.

\textbf{IDEA400} is a high-quality and expressive motion dataset recorded by ourselves, providing 13K motion sequences and 2.6M frames. Inheriting the NTU120~\cite{liu2019ntu} categories, we expand them to 400 actions with additional human self-contact motions, human-object contact motions, and expressive whole-body motions (e.g., rich facial expressions and fine-grained hand gestures). There are 36 actors with diverse appearance and clothing. For each action, we have the actors perform three times standing, three times walking, and four times sitting, a total of ten times. 
We annotate the SMPL-X format pseudo labels with the proposed motion annotation pipeline, which can generate high-quality whole-body motions. To obtain the semantic labels, we use the designed action labels and expand them with the large language model (LLM)~\cite{jiao2023chatgpt}. The pose descriptions are annotated with our whole-body pose captioning method. 
In this subset, we provide monocular videos, the body keypoints, SMPL-X parameters, and action labels. Please see the video on our website for more details and visualization. 

\textbf{UBC Fashion}~\cite{UBCdwnet} 
The UBC Fashion Dataset is a high-resolution dataset specifically designed for human video synthesis tasks. It contains 500 training videos and 100 test videos, with each video containing approximately 350 frames. The videos feature a single human subject in front of a static camera, and the dataset includes a diverse array of clothing and textures to cover a wide range of appearances. This makes it particularly useful for tasks that involve pose-guided human video generation.

\textbf{AIST}~\cite{tsuchida2019aist} is a large-scale dance dataset with multi-view videos and dance genre labels. Instead of using the body-only SMPL annotations from AIST++~\cite{li2021aist}, we annotate the whole-body motion via our motion annotation pipeline. We obtain the semantic labels by expanding the dance genre label and providing frame-level pose descriptions.

\textbf{HAA500}~\cite{chung2021haa500} is a large-scale human-centric atomic action dataset with manually annotated labels and videos for action recognition. It contains 500 classes with fine-grained atomic action labels, covering sports, playing musical instruments, and daily actions. However, it does not have the motion labels. We annotate the 3D whole-body motion with our pipeline. We use the provided atomic action label as semantic labels. Besides, we input the video into video-LLaMA~\cite{damonlpsg2023videollama} and filter the human action descriptions as supplemental texts. Pose description is generated by our automatic pose annotation method.

\textbf{HuMMan}~\cite{cai2022humman} is a human dataset with multi-modality data, including multi-view videos, keypoints, SMPL parameters, action labels, etc. It does not provide whole-body pose labels. We estimate the SMPL-X parameters with our annotation pipeline. Besides, we expand the action label with LLM into semantic labels and use the proposed captioning pipeline to obtain pose descriptions.

\textbf{GRAB}~\cite{taheri2020grab} is human grasping dataset with body and hand motion. Meanwhile, it provides text descriptions of each grasping motion without corresponding videos. Therefore, similar to AMASS, we extract facial expressions from BAUM to fill in the facial expressions. We use the provided text description as semantic labels and annotate pose descriptions based on the SMPL-X parameters.

\textbf{EgoBody}~\cite{zhang2022egobody} is a large-scale dataset capturing ground-truth 3D human motions in social interactions scenes. It provides high-quality body and hand motion annotations, lacking facial expression. Thus, we perform a motion augmentation to obtain expressive whole-body motions. Since EgoBody does not provide text information, we manually label the semantic description using the VGG Image Annotation (VIA)~\cite{dutta2019vgg} and annotate the pose description with the automatic pose captioning pipeline.

\textbf{BAUM}~\cite{baum} is a facial dataset with 1.4K audio-visual clips and 13 emotions. We annotate facial expressions from BAUM with the SOTA face reconstruction method EMOCA.

\textbf{Online Videos.} To improve the richness of appearance and motion diversity, especially on professional motions, we collect 33K monocular videos from online sources, covering various real-life scenes. We design action categories as motion prompts and input them into LLM. Then, we collect videos from online sources based on the answer of LLM, after which we filter the candidate videos by transition detection and annotate the whole-body motion, semantic label, and pose description for the selected videos.

\subsection{Motion Augmentation Mechanism}
\label{sec:motion_aug}

\noindent\textbf{Lower-body Motion Augmentation.} \dataname contains some upper-body videos collected from online videos, like the videos in UBody~\cite{osx}, where the lower-body part is invisible. Estimating accurate lower-body motions and global trajectories for these videos is challenging. Thanks to the precise low-body motions provided in AMASS, we can simply perform a lower-body motion augmentation for these sequences, i.e., selecting the closest motion from AMASS based on the SMPL-X parameters and replacing the lower-body motion with it. Meanwhile, we incorporate relevant keywords (e.g., sitting, standing, walking) in the text descriptions. Fig.~\ref{figure:motion_augmentation}(a) depicts three plausible lower-body augmentations for the motion sequence with the semantic label "a person is playing the guitar happily." 

\noindent\textbf{Facial Expression Augmentation.} As shown in Tab.~\ref{tab:statistic_subdataset}, the motion capture datasets AMASS, GRAB, and EgoBody do not provide facial expressions. Thus, we perform a facial expression augmentation for these motions by randomly selecting a facial expression sequence from the BAUM~\cite{baum} dataset to fill the void and incorporating emotion labels (e.g., happy, sad, and surprise) in the semantic description. We perform interpolation for the selected sequence to ensure the same length as the original motion. An example of face expression augmentation is illustrated in Fig.~\ref{figure:motion_augmentation}(b).

\subsection{Text caption promote}
Figure ~\ref{fig:text_promote}. shows the detailed caption promotes for GPT-4V in our text anntotation pipeline.
\begin{figure*}[h]	
    \centering
        \begin{center}
        \includegraphics[width=1\textwidth]{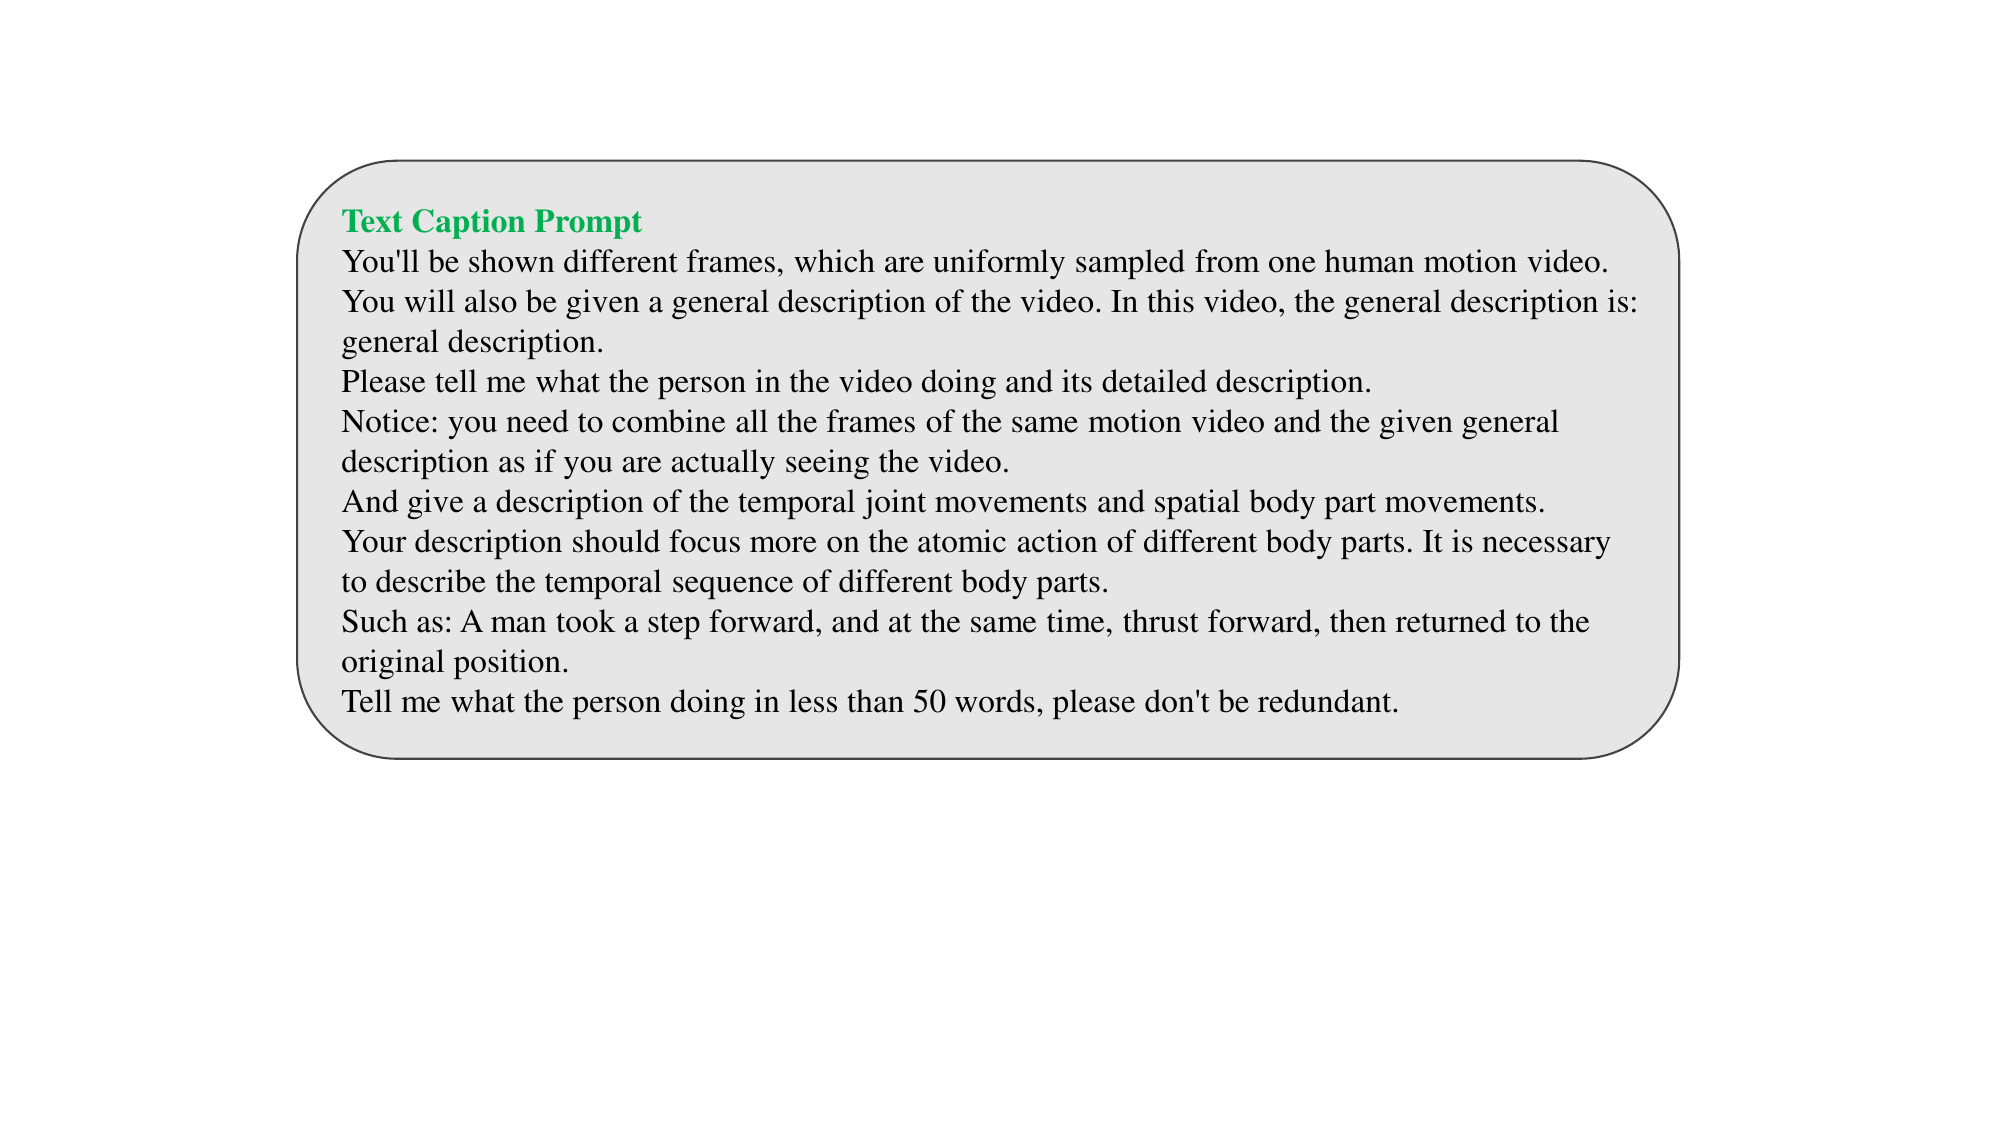}
    \end{center}

    \vspace{0.2cm}
    \caption{The detailed caption promotes for GPT-4V annotation process showed figure ~\ref{figure:overall_data_collection}.}
    \vspace{-0.4cm}
\label{fig:text_promote} 
\end{figure*}

\section{Experiment}
\subsection{Experiment Setup}

\label{sec:exp_detail}
\noindent \textbf{Motion Representation.} To capture the 3D expressive whole-body motion, we use SMPL-X~\cite{smpl-x} as our motion representation. A pose state is formulated as:
\begin{equation}
    \mathbf{x} = \{\theta_b, \theta_h, \theta_f, \psi, \mathbf{r} \}.
\end{equation}
Here, $\theta_b\in\mathbb{R}^{22\times3}$ and $ \theta_h\in\mathbb{R}^{30\times3}$ denote the 3D body rotations and hand rotations. $\theta_f\in \mathbb{R}^{3}$ and $\psi\in \mathbb{R}^{50}$ are the jaw pose and facial expression. $\mathbf{r}\in\mathbb{R}^3$ is the global translation.

\noindent \textbf{Evaluation Metrics.} We adopt the same evaluation metrics as \cite{humanml3d,guo2020action2motion}, including Frechet Inception Distance (FID), multimodality, diversity, R-precision, and multimodal distance. We pretrain a motion feature extractor and a text feature extractor for the new motion presentation with contrastive loss to map the text and motion into feature space and then evaluate the distance between the text-motion pairs. For each generated motion, its ground-truth text description and 31 mismatched text descriptions randomly selected from the test set compose a description pool. We rank the Euclidean distances between the generated motion and each text in the pool and then calculate the average accuracy at the top-k positions to derive R-precision. Multimodal distance is computed as the Euclidean distance between the feature vectors of generated motion and its corresponding text description in the test set. Additionally, We include the average temporal standard deviation as a supplementary metric to evaluate the diversity and temporal variation of whole-body motion.

\noindent \textbf{Computational Costs.} We use 8 NVIDIA A100 GPUs for motion annotation and 4 GPUs for motion generation experiments. It takes about 72 hours to annotate 1M frames with our annotation pipeline. 

\subsection{More Ablation Study}
\noindent\textbf{More Comparisons with HumanML3D.} 
Previous motion generation datasets are limited in expressing rich hand and face motions, as they only contain body and minimal hand movements. To demonstrate the expressiveness of our dataset, we conduct a comparison between HumanML3D and \dataname on face, hand, and body, separately. Specifically, we train MLD~\cite{mld} on each dataset and evaluate the diversity of generated and ground-truth motions by computing the average temporal standard deviation of the SMPL-X parameters and joint positions. 
The SMPL-X parameters include body poses, hand poses, and facial expressions. Body, hand, and face joint positions are represented as root-relative, wrist-relative, and neck-relative, respectively. We randomly choose 300 generated samples from the validation set and repeated the experiment 10 times to report the average results. As shown in Tab.~\ref{tab:ablation_motion}, the generated and ground-truth motions in \dataname exhibit a higher deviation, especially in hand and face parameters, indicating significant hand and face movements over time. These results demonstrate that the model trained with \dataname can generate more diverse facial expressions and hand motions, demonstrating the ability of our whole-body motion to capture fine-grained hand and face movements and expressive actions.  

\begin{table*}[h]
	\vspace{4pt}
        \centering
	\resizebox{0.6\textwidth}{!}{%
    \begin{tabular}{l|ccc|ccc}
        \toprule
        \multicolumn{1}{c|}{\multirow{2}[4]{*}{{Method}}} & \multicolumn{3}{c|}{\boldmath{}{Joints Position $\uparrow$}\unboldmath{}} & \multicolumn{3}{c}{\boldmath{}{SMPL-X Param ($10^{-2}$) $\uparrow$}\unboldmath{}} \\
        \cmidrule{2-7}
        & {Face} & {Hand} & {Body} & {Face} & {Hand} & {Body} \\
        \midrule
        HumanML3D (GT) & 0.00 & 0.00 & 88.7 & 0.00 & 0.00 & 9.01  \\
        Motion-X++ (GT) & 1.60 & 8.82 & 92.2 & 13.4 & 5.24 & 9.95  \\
        \midrule
        HumanML3D &0.00 & 0.00 & 64.8 & 0.00 & 0.00 & 7.23  \\
        Motion-X++ & 1.33 & 11.4 & 66.0 & 7.28 & 5.30 & 7.41  \\
        \bottomrule
        \end{tabular}
	}
    \caption{\small Temporal standard deviation of the SMPL-X parameters and joint positions on HumanML3D and \dataname. We compare the GT and generated motions with the MLD model trained on HumanML3D and \dataname, respectively.}	       
    \label{tab:ablation_motion}
\vspace{-0.3cm}
\end{table*}
\noindent\textbf{Ablation Study with different subset in \newdataname}
On Tab.~\ref{tab:rtmpose_supp}(a), we identified subsets that are likely to have a positive impact on rtmpose training. Notably, apart from the fitness and kungfu subsets in our dataset, this conclusion aligns with our understanding of the data. In the subsets that do not positively contribute to training, the input videos feature very few actors, which may lead to biased training results. In the second Tab.~\ref{tab:rtmpose_supp}(b), we adjusted the input video downsampling rate for this single-frame algorithm to reduce redundancy in the training data while maintaining a consistent overall data volume. The proportions of the different datasets were set to \newdataname :CoCo\-Wholebody:Ubody = $2:1:1.5$.
\begin{figure*}[h]
  \centering
  % Table a
  \subfloat[\small Ablation study on different subset in \newdataname.]{
    \resizebox{\textwidth}{!}{
      \begin{tabular}{l|cc|cc|cc|cc|cc}
        \toprule
        
        \rowcolor{lightgray}
        \multirow{2}{*}{} & \multicolumn{2}{c|}{Body $\uparrow$} &
                           \multicolumn{2}{c|}{Foot $\uparrow$} & 
                           \multicolumn{2}{c|}{Face $\uparrow$} & 
                           \multicolumn{2}{c|}{Hand $\uparrow$} & 
                           \multicolumn{2}{c}{Wholebody $\uparrow$} \\
        \rowcolor{lightgray}
        \multirow{-2}{*}{Training data} & AP & AR & AP & AR & AP & AR & AP & AR & AP & AR \\
        \midrule
        Ubody+COCO(baseline) & 0.492 & 0.579 & 0.332 & 0.508 & 0.703 & 0.787 & 0.328 & 0.460 & 0.409 & 0.503 \\
        Ubody+COCO+haa500 & \textbf{0.521} & \textbf{0.604} & \textbf{0.426} & \textbf{0.596} & \textbf{0.704} & 0.784 & \textbf{0.328} & \textbf{0.462} & \textbf{0.428} & \textbf{0.523} \\
        Ubody+COCO+animation & 0.503 & 0.590 & 0.365 & 0.541 & 0.695 & 0.777 & 0.314 & 0.449 & 0.413 & 0.507 \\
        Ubody+COCO+humman & 0.497 & 0.585 & 0.380 & 0.560 & 0.689 & 0.774 & 0.320 & 0.452 & 0.411 & 0.505 \\
        Ubody+COCO+music & 0.494 & 0.582 & 0.338 & 0.517 & 0.698 & 0.777 & 0.310 & 0.442 & 0.406 & 0.501 \\
        Ubody+COCO+perform & 0.503 & 0.591 & 0.377 & 0.556 & 0.693 & \textbf{0.779} & 0.325 & 0.459 & 0.414 & 0.509 \\
        Ubody+COCO+kungfu & 0.449 & 0.540 & 0.310 & 0.491 & 0.672 & 0.746 & 0.258 & 0.398 & 0.365 & 0.459 \\
        Ubody+COCO+IDEA400 & 0.500 & 0.586 & 0.412 & 0.583 & 0.696 & 0.777 & 0.330 & 0.468 & 0.416 & 0.510 \\
        Ubody+COCO+fitness & 0.489 & 0.575 & 0.378 & 0.554 & 0.684 & 0.768 & 0.313 & 0.443 & 0.402 & 0.494 \\
        \bottomrule
      \end{tabular}
    }
  }
  
  % \hfill
  % Table b
  \subfloat[\small Ablation study on different data down sample rate.]{
    \resizebox{\textwidth}{!}{
      \begin{tabular}{c|cc|cc|cc|cc|cc}
        \toprule
        \rowcolor{lightgray}
        \multirow{2}{*}{} & \multicolumn{2}{c|}{Body $\uparrow$} &
                           \multicolumn{2}{c|}{Foot $\uparrow$} &
                           \multicolumn{2}{c|}{Face $\uparrow$} &
                           \multicolumn{2}{c|}{Hand $\uparrow$} &
                           \multicolumn{2}{c}{Wholebody $\uparrow$} \\
        \rowcolor{lightgray}
        \multirow{-2}{*}{Down sample rate} & AP & AR & AP & AR & AP & AR & AP & AR & AP & AR \\
        \midrule
        1 & 0.492 & 0.579 & 0.332 & 0.508 & 0.703 & 0.787 & 0.328 & 0.460 & 0.409 & 0.503 \\
        3 & \textbf{0.521} & \textbf{0.604} & \textbf{0.426} & \textbf{0.596} & \textbf{0.704} & 0.784 & \textbf{0.328} & \textbf{0.462} & \textbf{0.428} & \textbf{0.523} \\
        5 & 0.503 & 0.590 & 0.365 & 0.541 & 0.695 & 0.777 & 0.314 & 0.449 & 0.413 & 0.507 \\
        7 & 0.497 & 0.585 & 0.380 & 0.560 & 0.689 & 0.774 & 0.320 & 0.452 & 0.411 & 0.505 \\
        \bottomrule
      \end{tabular}
    }
  }
  % \hfill 
  \caption{\small Ablation experiments for training whole-body pose estimation using \newdataname data evaluate on COCO-Wholebody ~\cite{coco_wholebody}, we evaluated the impact of using different subsets and various downsampling rates on the training performance.} 
  \label{tab:rtmpose_supp}
  \vspace{-0.2in}
\end{figure*}

\subsection{Music-Driven Motion Generation Results}
\begin{figure*}[h]
    \begin{center}
        \includegraphics[width=1\textwidth]{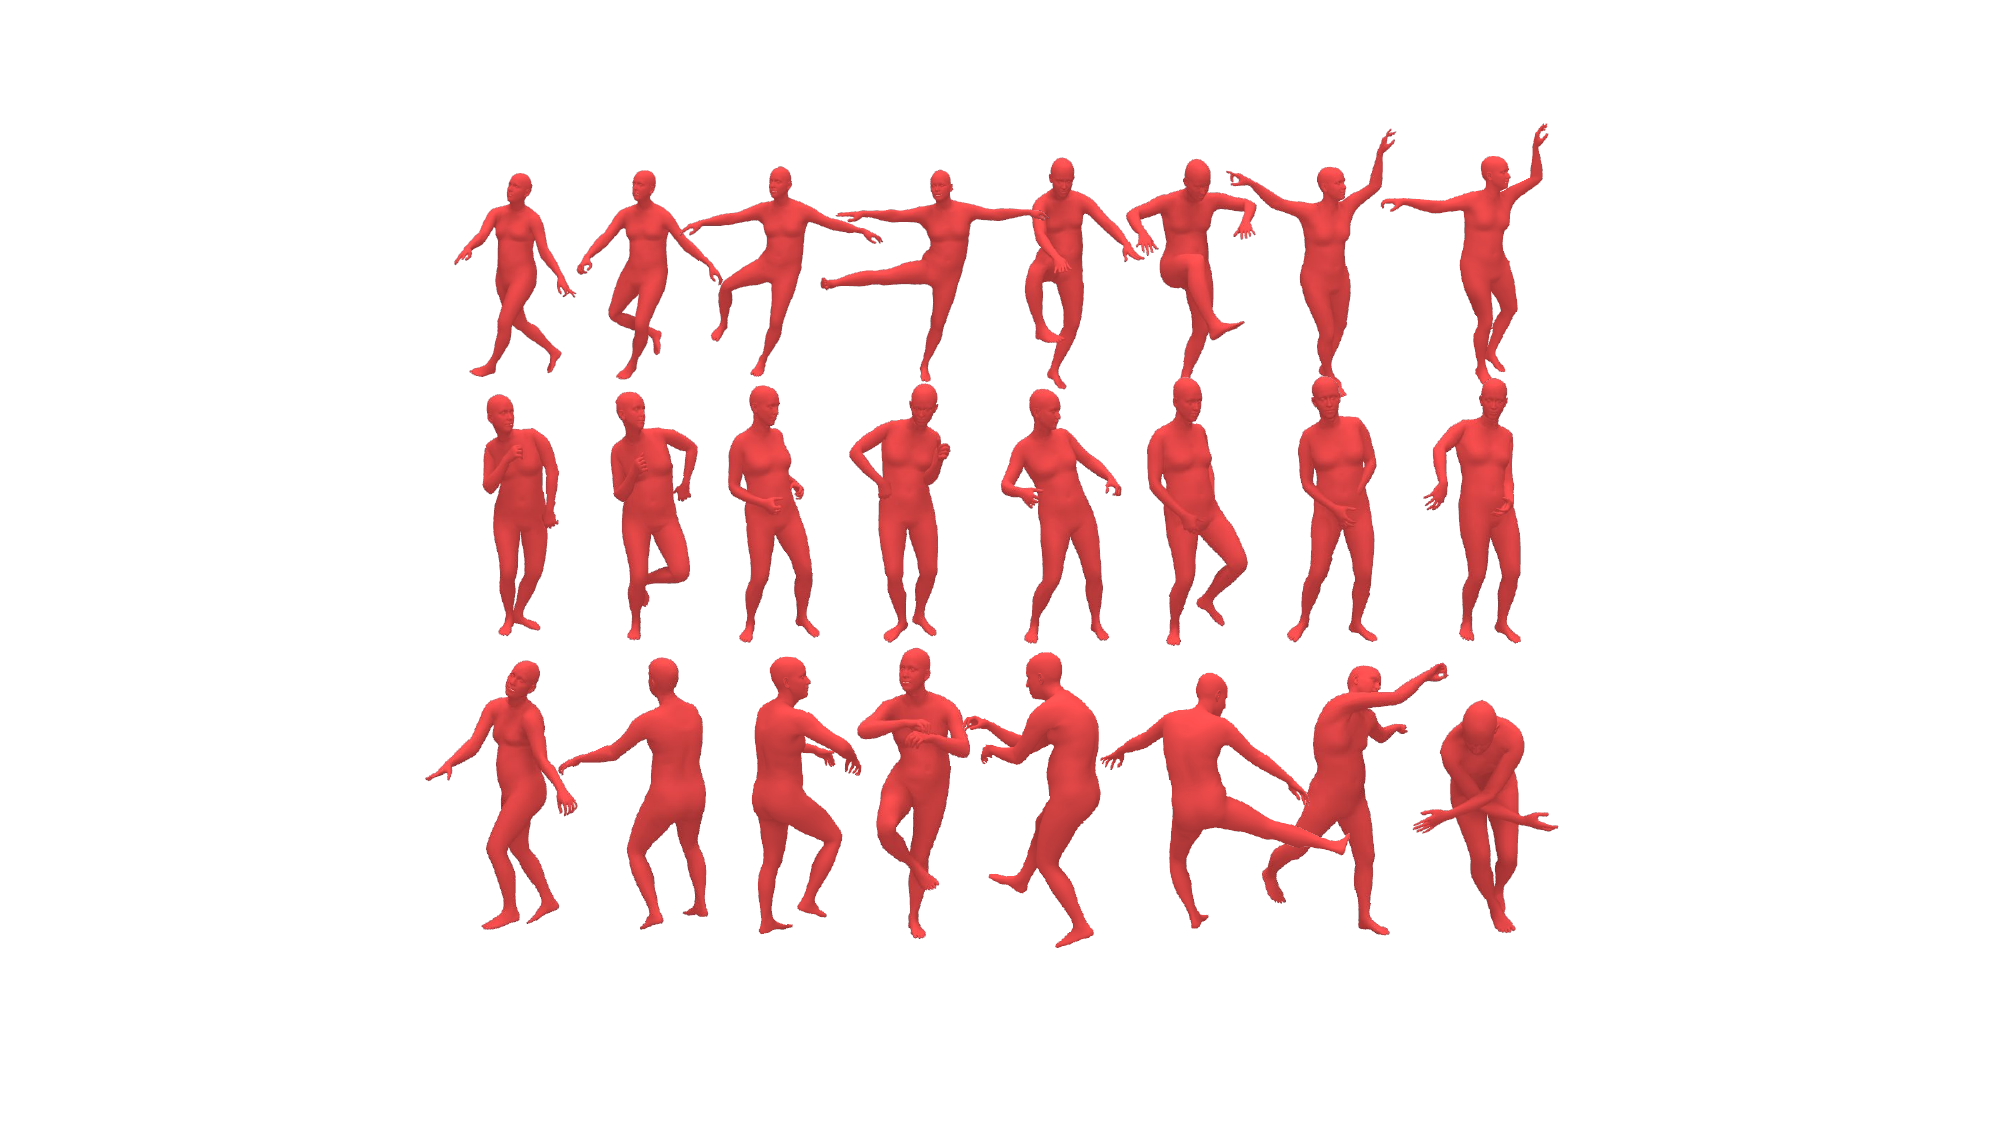}
    \end{center}
    % \vspace{-0.6cm}
    \caption{Audio driven motion generation results (Trained on \newdataname data.)}
    \label{figure:dance}
\end{figure*}
In figure~\ref{figure:dance}, we show some results of music-driven motion generation trained with \newdataname data.
The ~\cite{finedance} model trained on \newdataname demonstrates a remarkable capacity to generate diverse and naturalistic dance motions. These generated movements not only adhere to physical constraints but also effectively mitigate the common foot sliding artifacts.

\section{More Annotation Visual Results}
In this section, we present some visual results of the 2D keypoints, SMPL-X parameters, and motion sequences to show the effectiveness of our proposed motion annotation pipeline. 

\subsection{2D Keypoints}
As the main paper claims, we propose a hierarchical Transformer-based model for 2D keypoints estimation. To demonstrate the superiority of our method, we compare it with two widely used methods, Openpose~\cite{openpose} and MediaPipe~\cite{mediapipe}. We use the PyTorch implementation of Openpose and only estimate the body and hand keypoints as it does not provide the face estimator. As shown in Fig.~\ref{figure:kpt_annot_compare}, Openpose and MediaPipe can not achieve accurate results in some challenging poses. Besides, there exists severe missing detection of hands for Openpose and MediaPipe. In contrast, our method performs significantly better, especially the hand keypoint localization.

\subsection{SMPL-X Parameters}
To register accurate SMPL-X parameters, we elaborately design a learning-based fitting method with several training loss functions. We compare our method with two SOTA learning-based methods, Hand4Whole~\cite{GyeongsikMoon2020hand4whole} and OSX~\cite{osx}. As shown in Fig.~\ref{figure:smplx_annot_compare}, our method achieves a much better alignment result than the other models, especially on some difficult poses, which benefits from the iterative fitting process. Notably, Hand4Whole~\cite{GyeongsikMoon2020hand4whole} and OSX~\cite{osx} can only estimate the local positions without optimized global positions, which will suffer from unstable and jittery global estimation.
Furthermore, we compare with the widely used fitting method SMPLify-X~\cite{smpl-x}, using their officially released codes, in Fig.~\ref{figure:comp_smplyx}. Our method is more robust than SMPLify-X and can obtain better results about physically plausible poses, especially in challenging scenes (e.g., hard poses, low-resolution inputs, heavy occlusions). The results from the side view demonstrate that our method can properly deal with depth ambiguity and avoid the lean issue.

\subsection{Motion Sequences}
To highlight the expressiveness and diversity of our proposed motions, we illustrate examples of the same semantic label, like \emph{dance ballet}, with six motion styles in Fig.~\ref{figure:ballet}. This one-to-many (text-to-motion) information can benefit the diversity of motion generation.
Then, we demonstrate more motion visualization in Fig.~\ref{figure:supp_viz1} and \ref{figure:supp_viz2} for different motion scenes. These motions show different facial expressions, hand poses, and body motions. 

% \clearpage

\begin{figure*}[h]
    \begin{center}
        \includegraphics[width=1\textwidth]{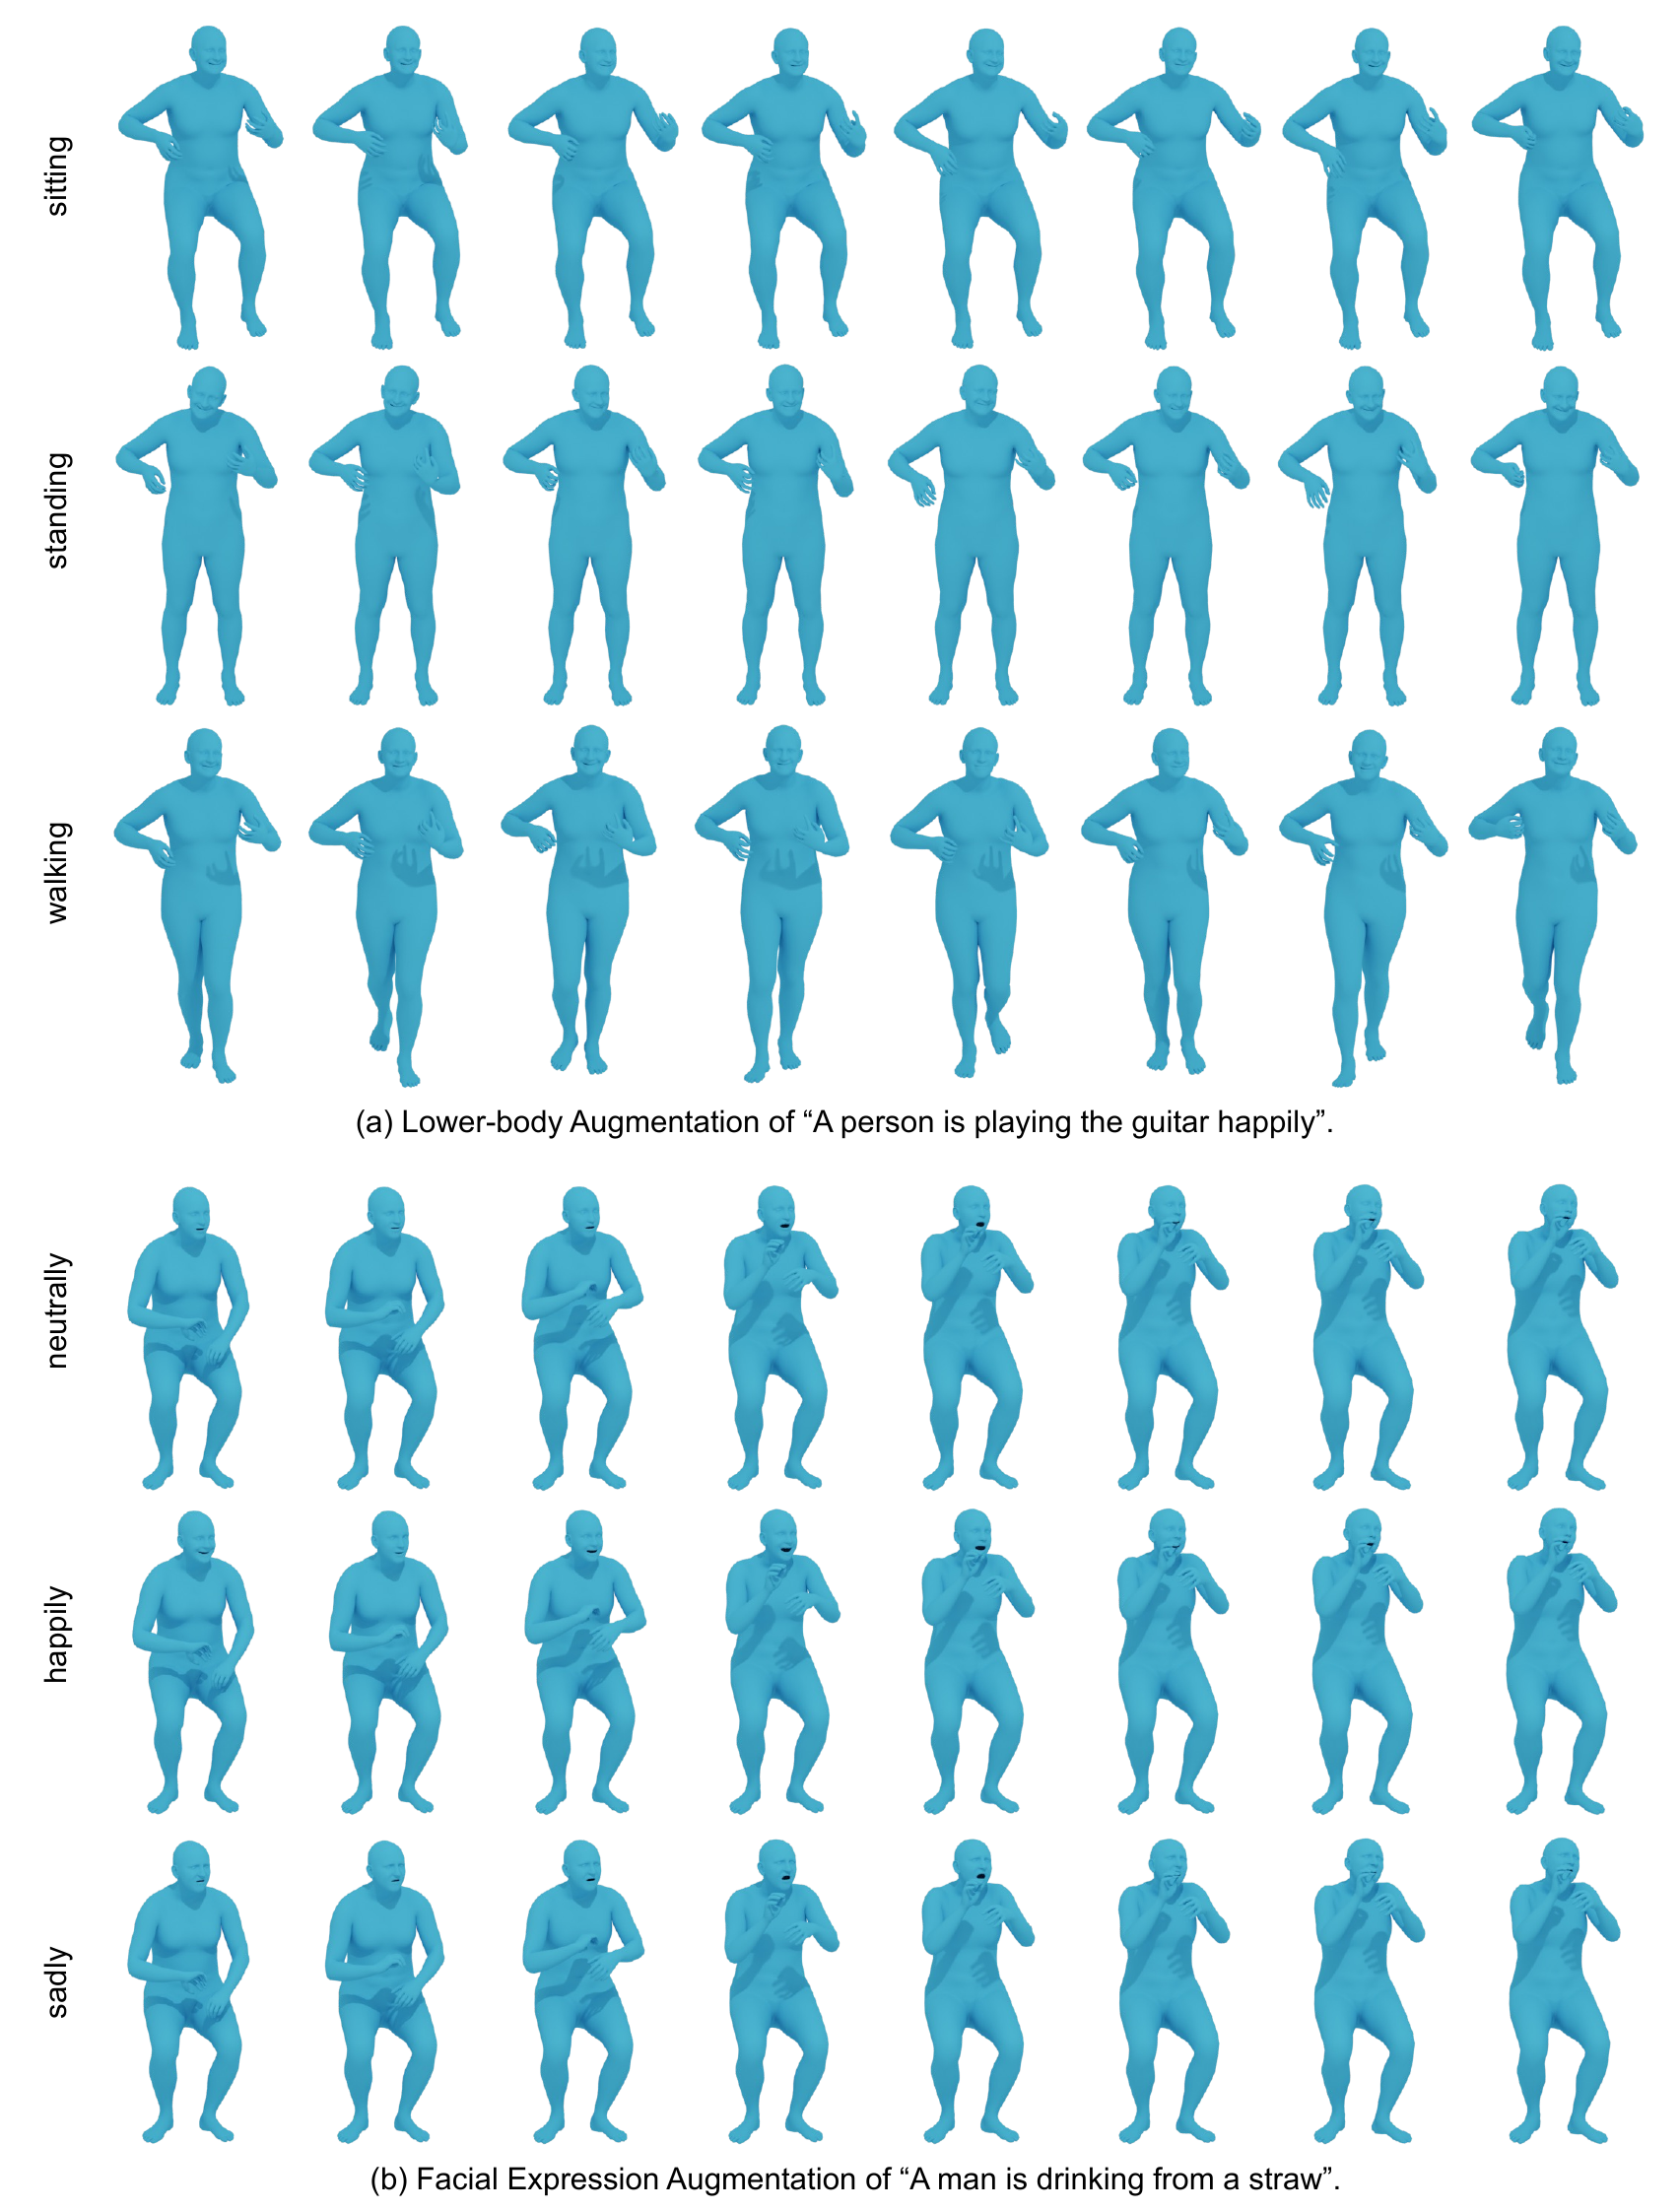}
    \end{center}
    % \vspace{-0.6cm}
    \caption{Illustration of two motion augmentation methods: (a) lower-body augmentation. (b) facial expression augmentation.}
    \label{figure:motion_augmentation}
\end{figure*}
    
\begin{figure*}[h]
    \begin{center}
        \includegraphics[width=1\textwidth]{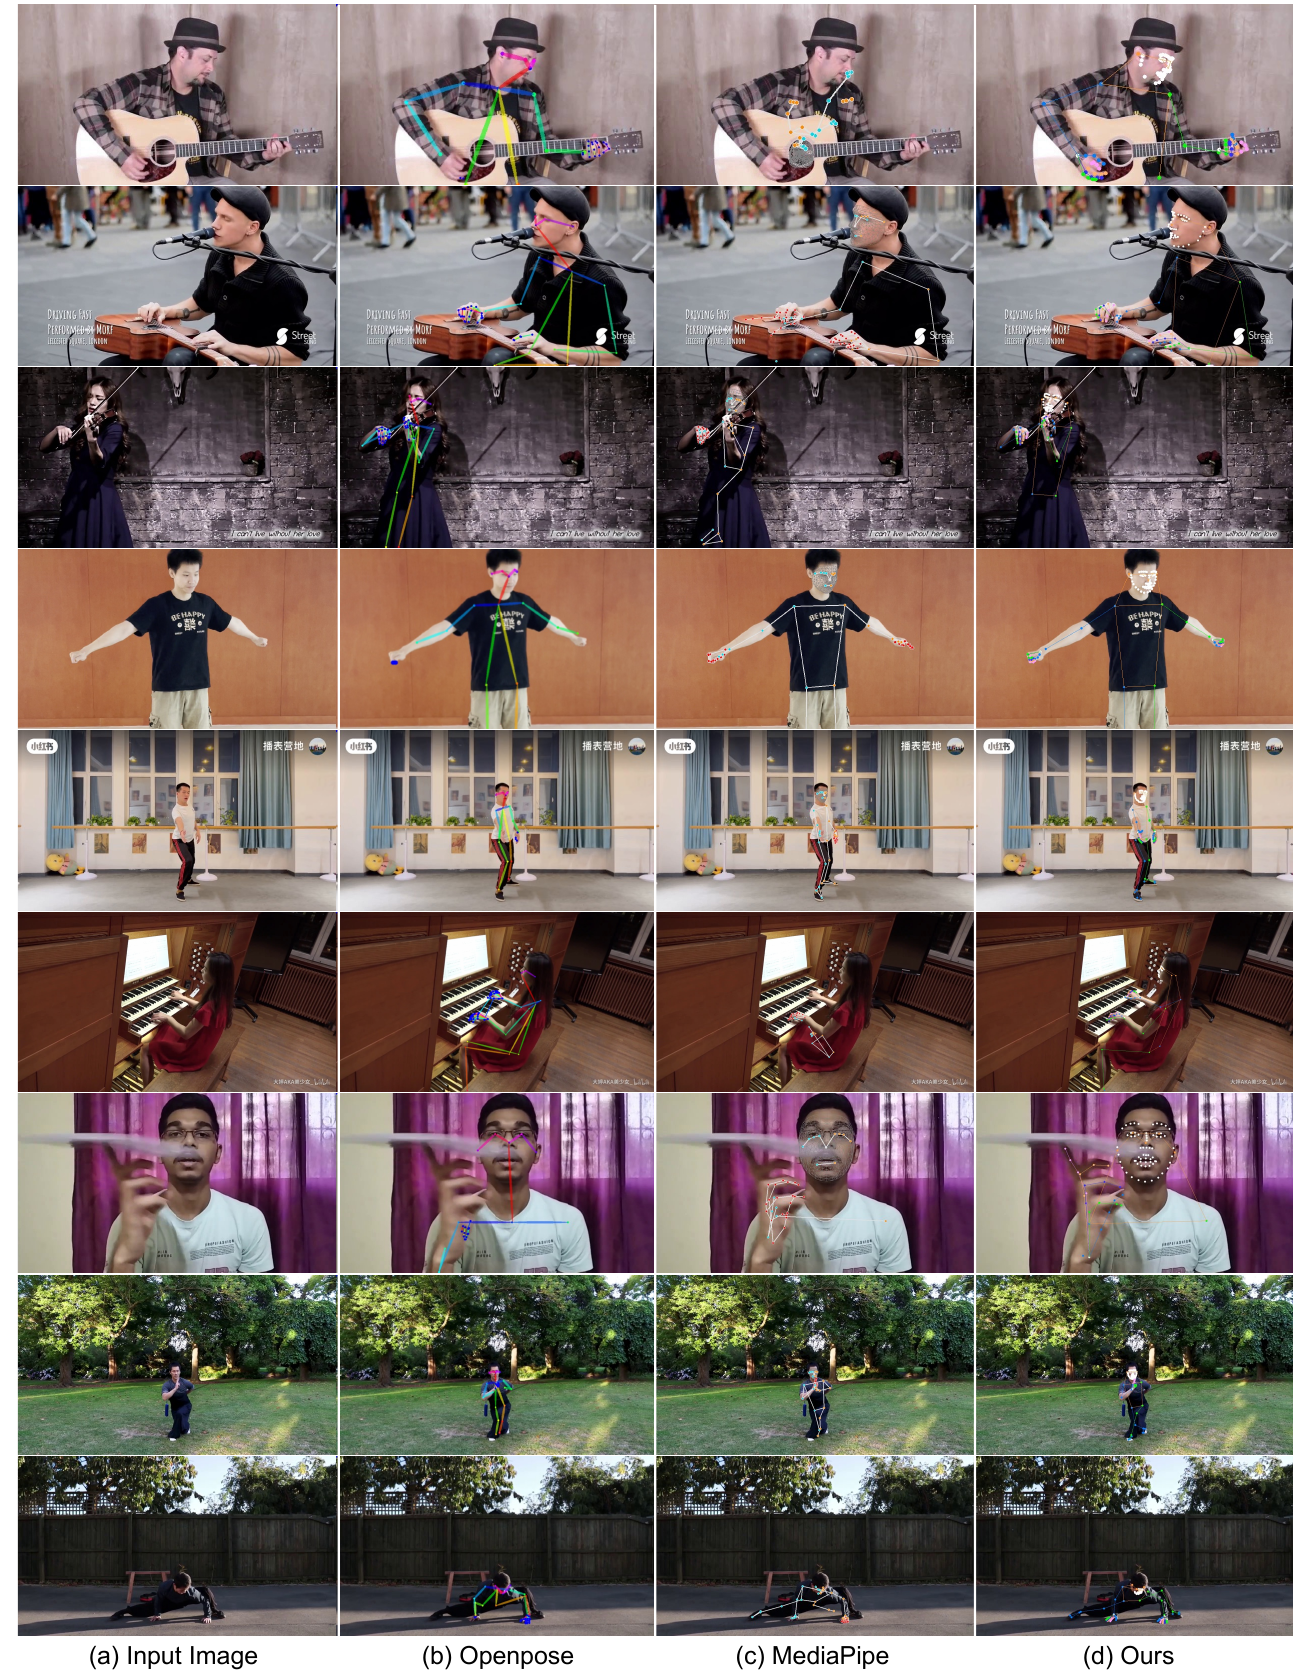}
    \end{center}
    % \vspace{-0.6cm}
    \caption{Comparisons of the 2D keypoints annotation quality with widely used methods Openpose~\cite{openpose} and MediaPipe~\cite{mediapipe}.}
    \label{figure:kpt_annot_compare}
    \end{figure*}
    
    \begin{figure*}[h]
    \begin{center}
        \includegraphics[width=1\textwidth]{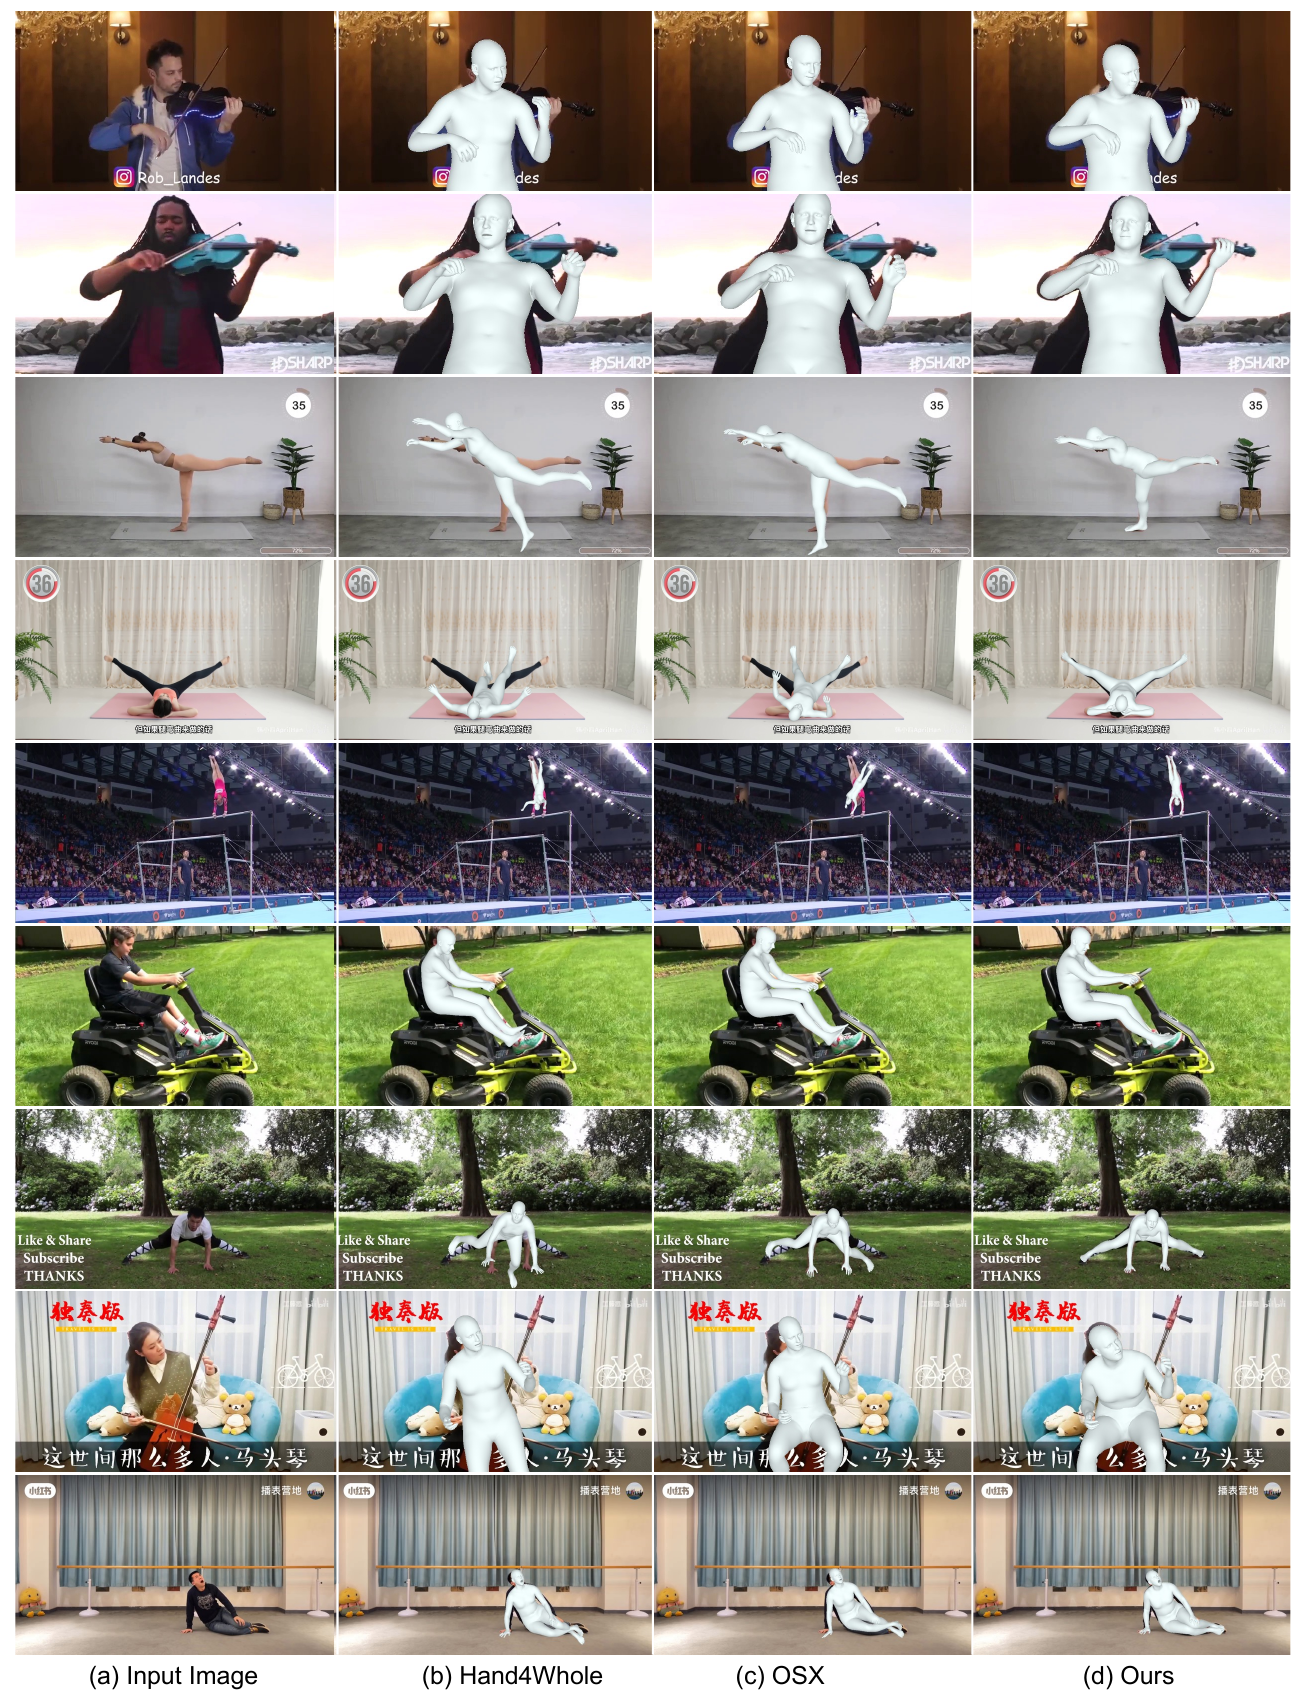}
    \end{center}
    \caption{Comparisons of the 3D SMPL-X annotation quality with SOTA methods Hand4Whole~\cite{GyeongsikMoon2020hand4whole} and OSX~\cite{osx}.}
    \label{figure:smplx_annot_compare}
    \end{figure*}

    \begin{figure*}[h]
    \begin{center}
        \includegraphics[width=1\textwidth]{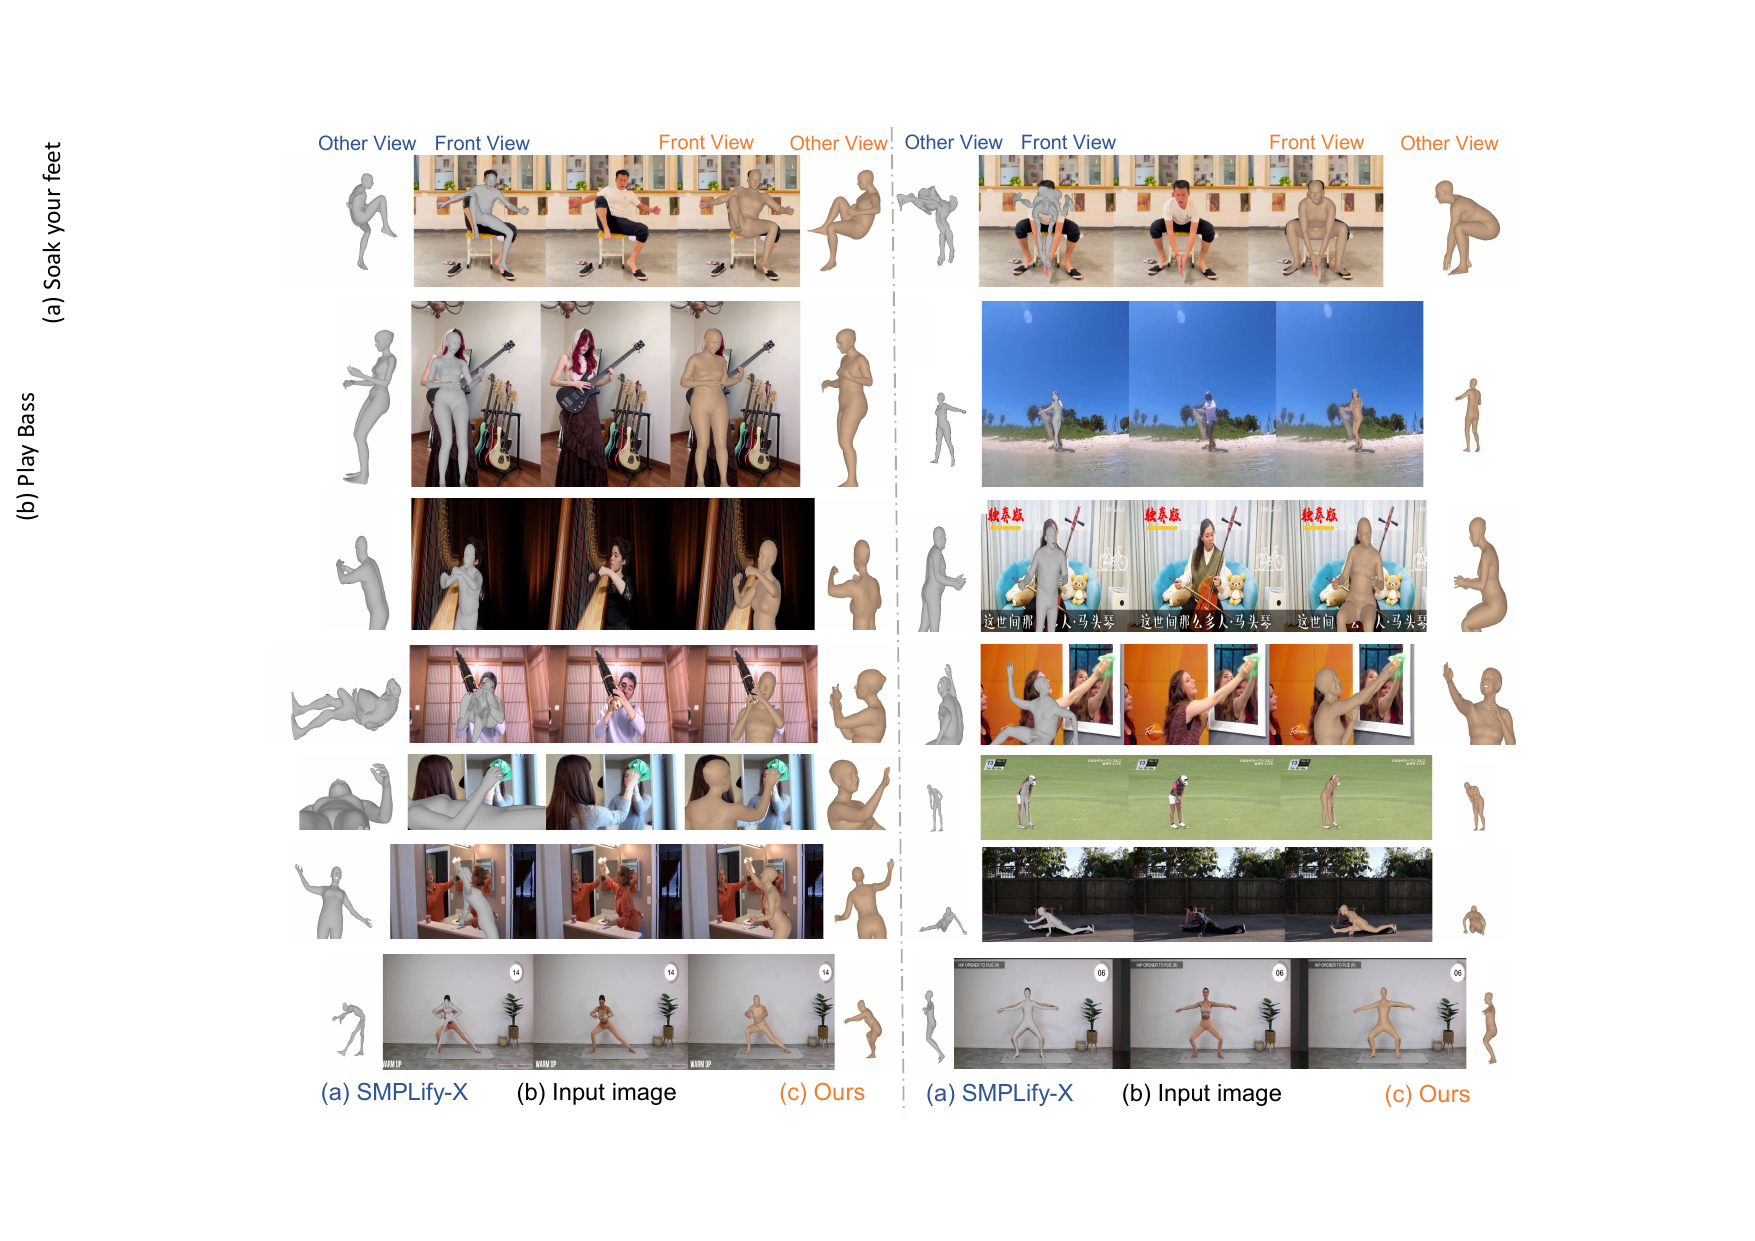}
    \end{center}
    \caption{Comparisons of the 3D SMPL-X annotation quality with wide-used fittiing methods SMPLify-X~\cite{smpl-x}.}
    \label{figure:comp_smplyx}
    \end{figure*}

    \begin{figure*}[h]
    \begin{center}
        \includegraphics[width=1\textwidth]{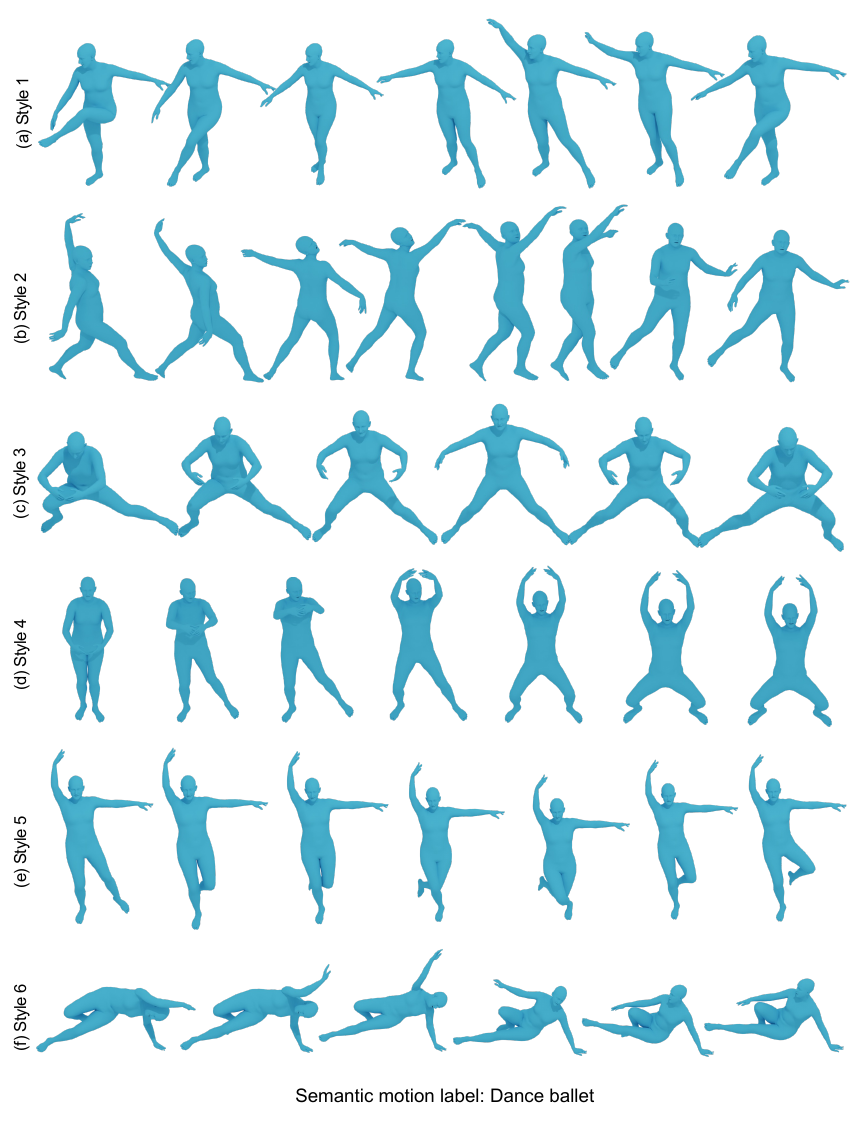}
    \end{center}
    \caption{Examples of the same semantic label ``dance ballet'' with different styles to enhance the motion diversity.}
    \label{figure:ballet}
    \end{figure*}
    
    \begin{figure*}[h]
    \begin{center}
        \includegraphics[width=1\textwidth]{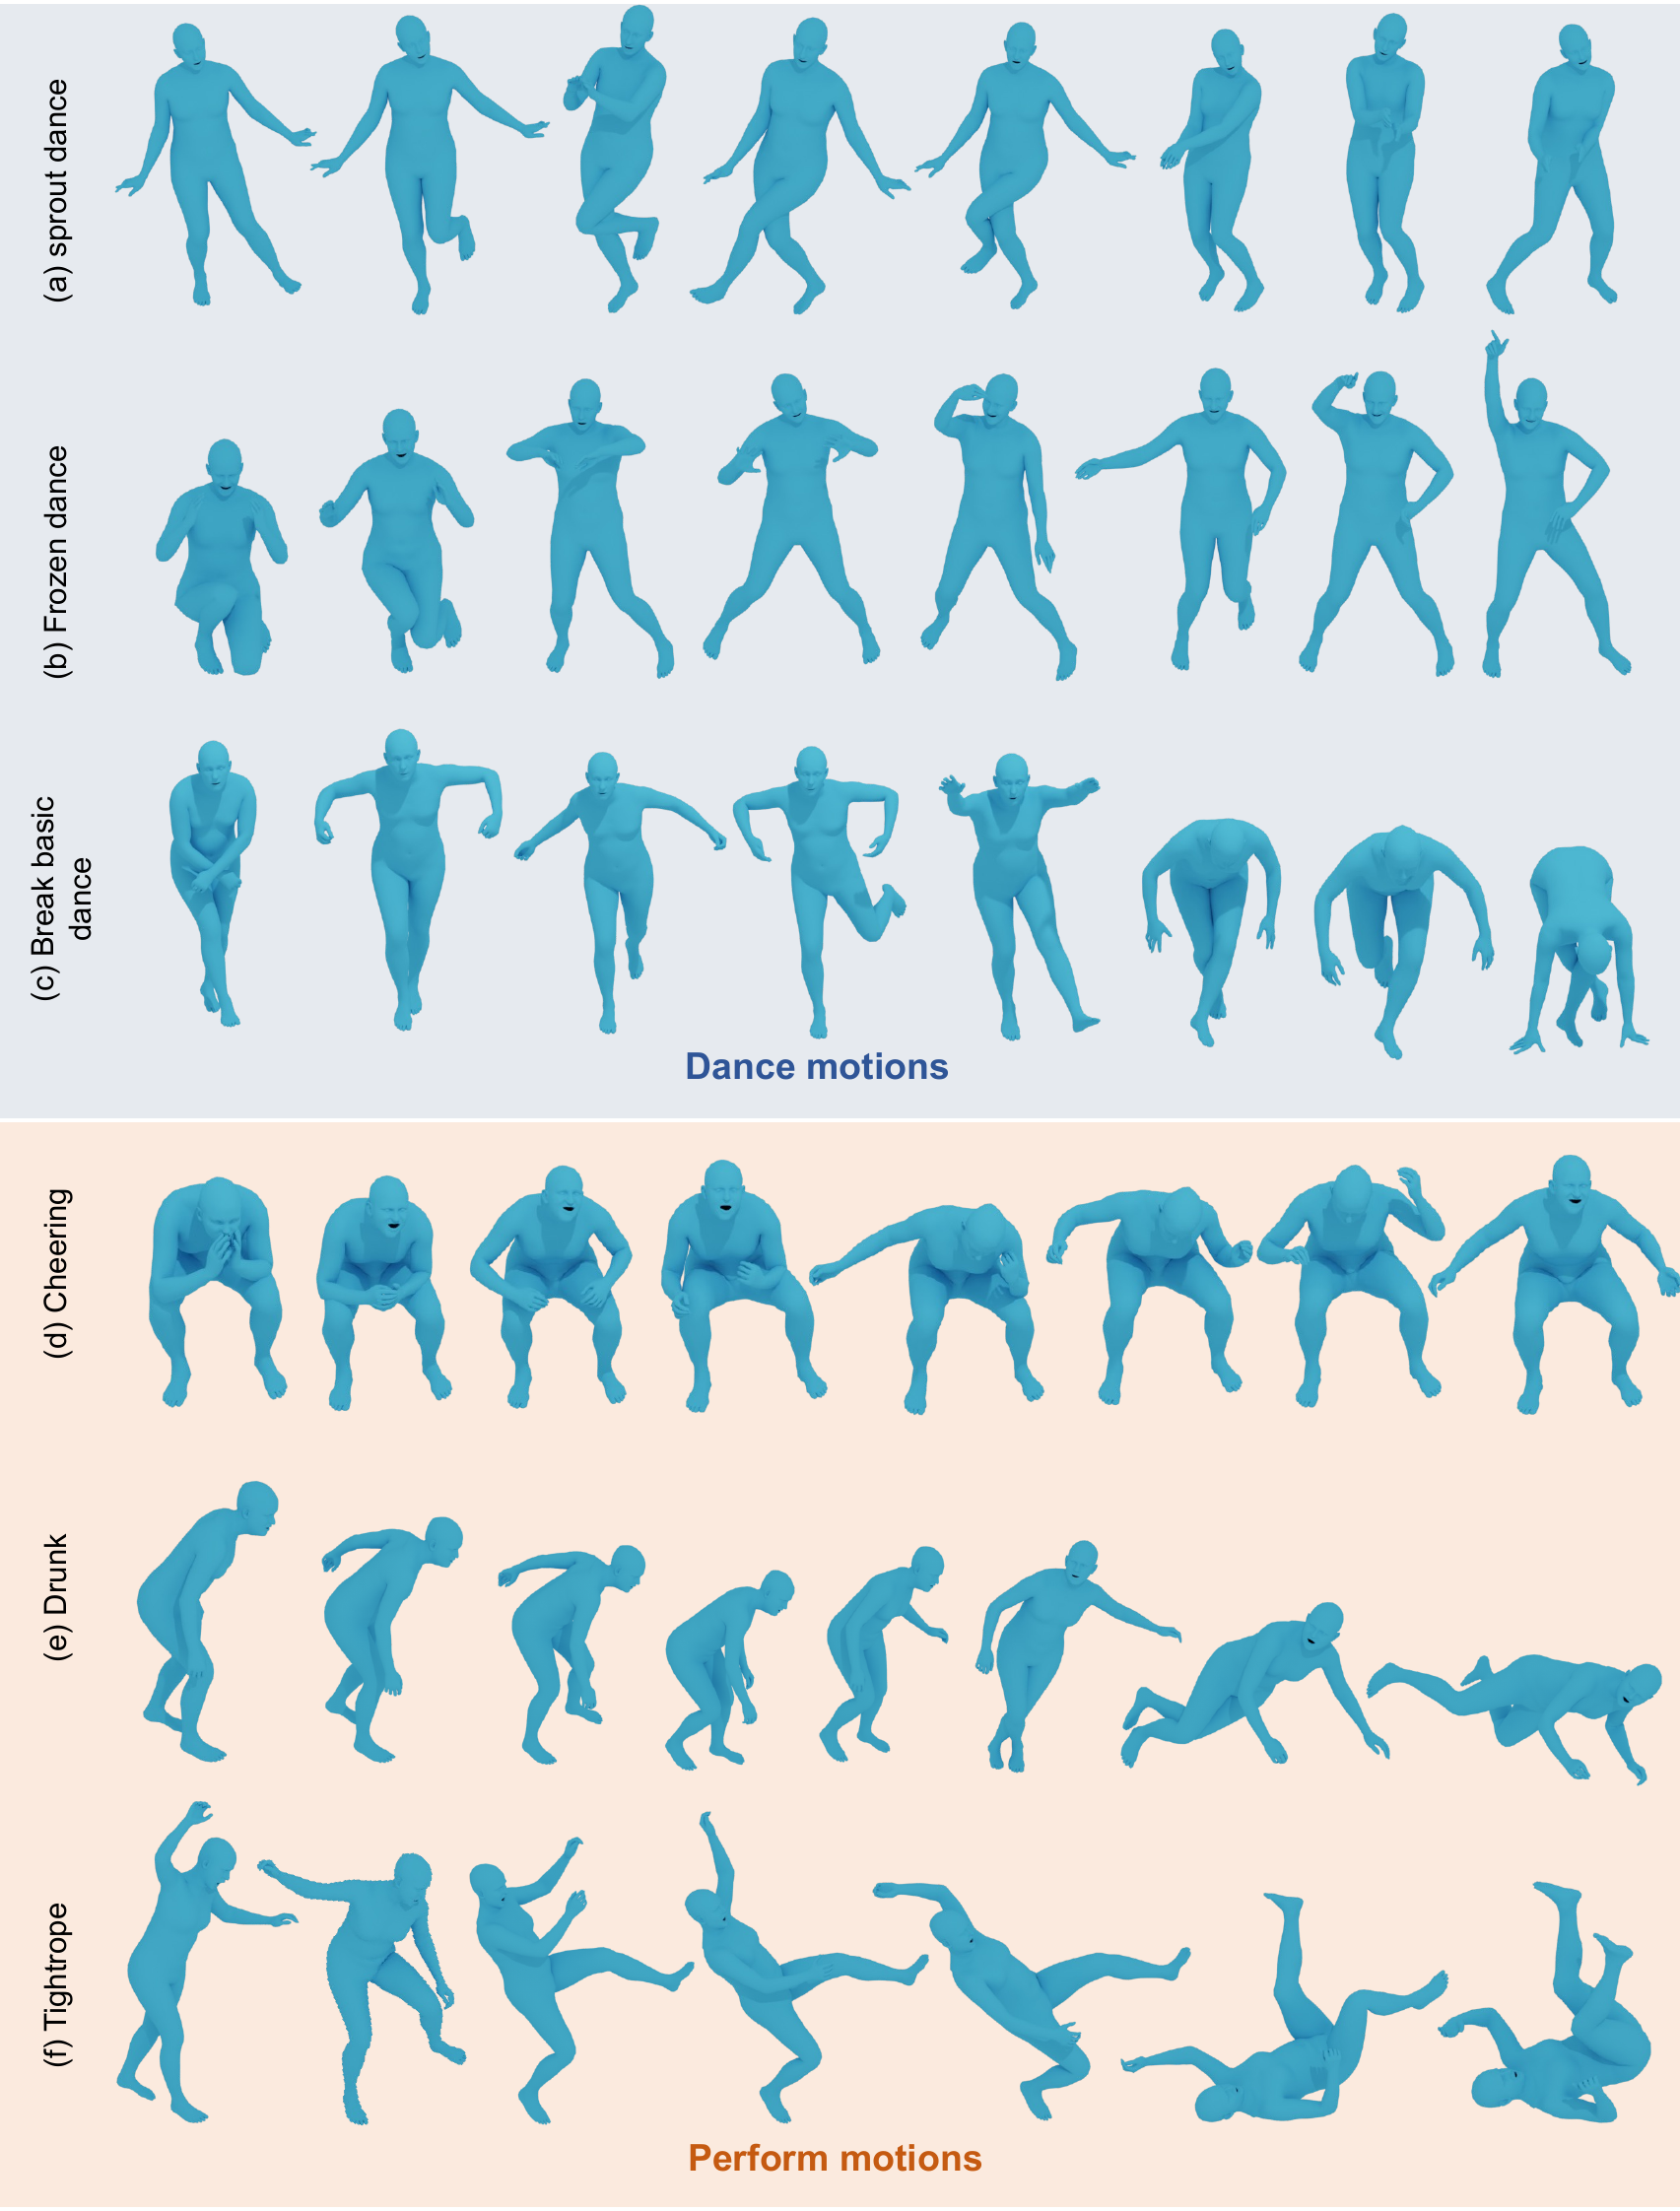}
    \end{center}
    \caption{Visualization of the dance and perform motion sequences of \dataname.}
    \label{figure:supp_viz1}
    \end{figure*}
    
    \begin{figure*}[h]
    \begin{center}
        \includegraphics[width=1\textwidth]{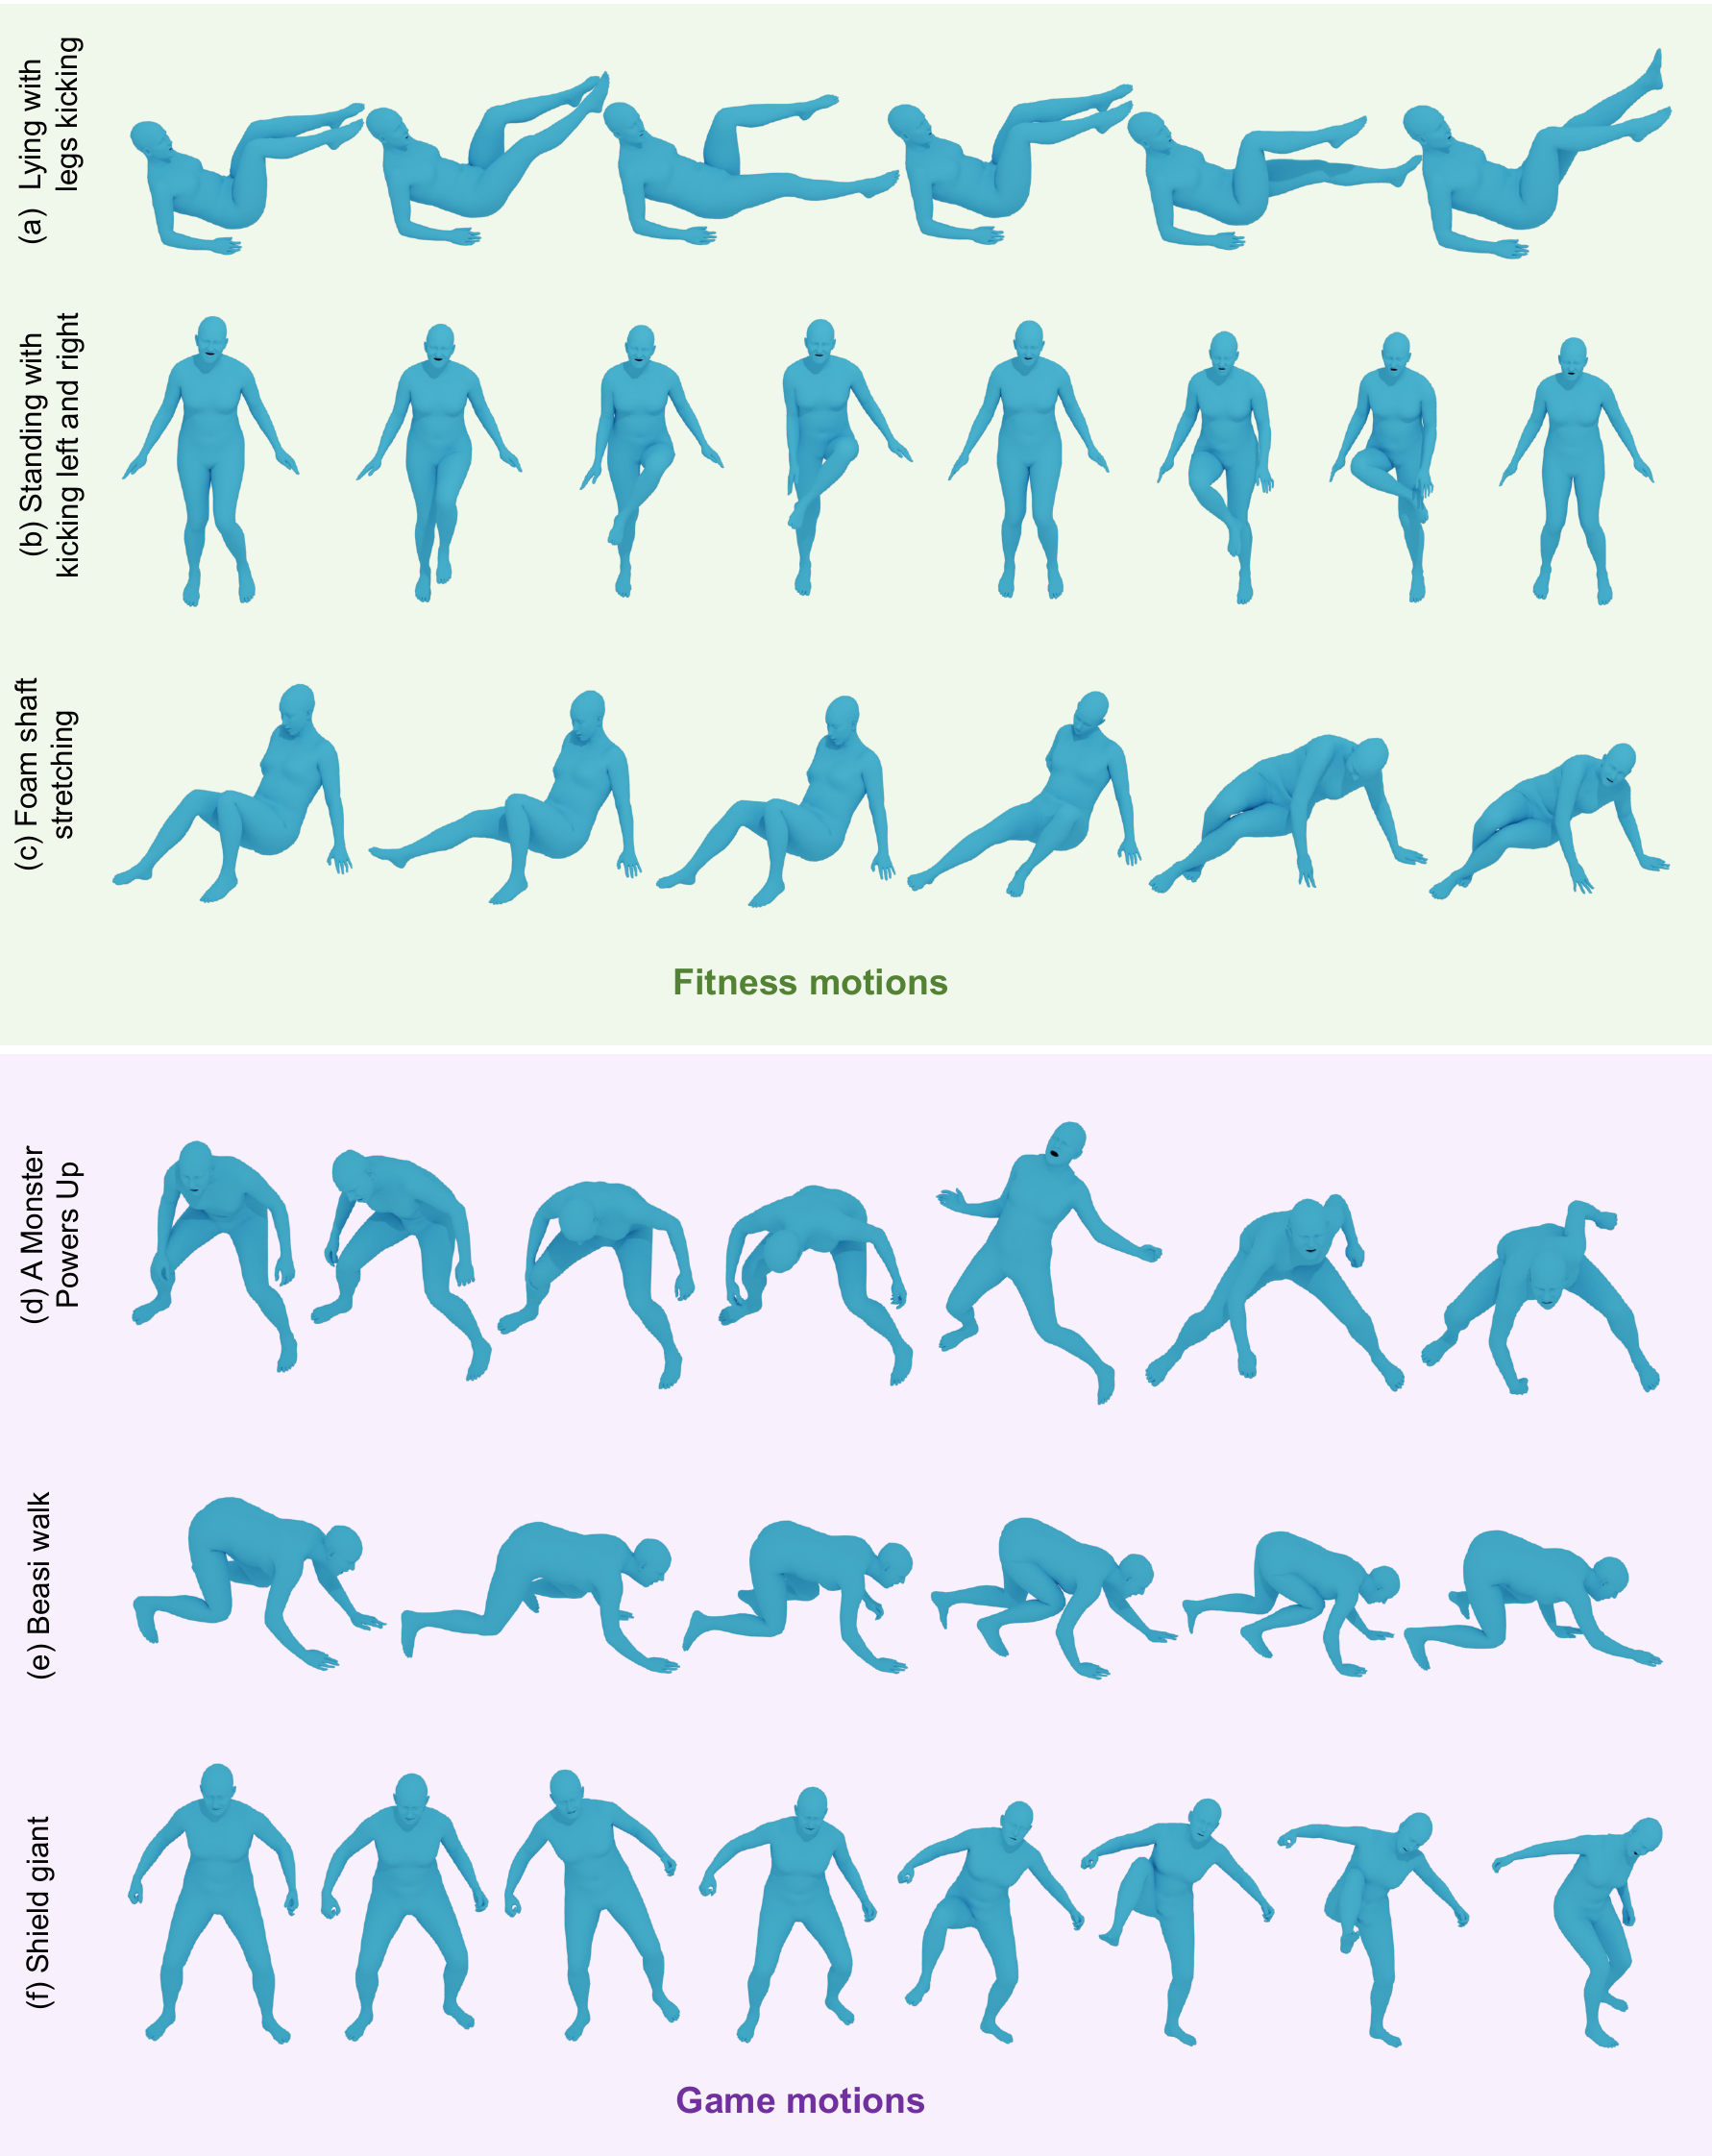}
    \end{center}
    \caption{Visualization of the fitness and game motion sequences of \dataname.}
    \label{figure:supp_viz2}
    \end{figure*}

\section{Related Work}

In this part, we introduce relevant \textbf{methods} for human motion generation.

According to different inputs, producing human motions can be divided into two categories: the general motion synthesis from scratch~\cite{yan2019convolutional,zhao2020bayesian,zhang2020perpetual,cai2021unified} and the controllable motion generation from given text, audio, and music as conditions~\cite{ahn2018text2action,temos,modiff,motiondiffuse,mld,humanml3d,ahuja2019language2pose,ghosh2021synthesis}. 
Motion synthesis encompasses several tasks, such as motion prediction, completion, and interpolation~\cite{cai2021unified}, developed over several decades in computer vision and graphics. These tasks tend to utilize nearby frames with spatio-temporal correlations to infer estimated frames in a deterministic manner~\cite{martinez2017human,butepage2017deep,cai2020learning,fragkiadaki2015recurrent,ghosh2017learning,kaufmann2020convolutional,mao2019learning,mao2020history}. 
On the other hand, motion generation is a more challenging task that aims to synthesize long-term, diverse, natural human motions. 

Many generative models, like GANs, VAEs, and recent diffusion models, have been explored~\cite{wang2020learning,yu2020structure,action2video,guo2020action2motion,petrovich2021action}.
This work mainly discusses text-conditioned motion generation. This field has evolved from inputting action classes~\cite{action2video,guo2020action2motion} to sentence descriptions~\cite{humanml3d,mld,motiondiffuse}, and generating motions from 2D to 3D keypoints, to the emerging parametric model (e.g., SMPL~\cite{smpl,humanml3d,mld}). These models have become expressive and comprehensive toward real-world scenarios thanks to the development of related benchmarks. 
Recently, diffusion model-based methods have rapidly developed and shown advantages in diverse, realistic, and fine-grained motion generation~\cite{motiondiffuse,mld,modiff,Tevet2022HumanMD,Yuan2022PhysDiffPH}. Some concurrent works~\cite{Tevet2022HumanMD,motiondiffuse,mld} introduce novel diffusion model-based motion generation framework to achieve state-of-the-art (SOTA) quality. For example, MLD~\cite{mld} presents a motion latent-based diffusion model with a representative motion variational autoencoder, showing its efficiency. Based on the proposed Motion-X, HumanTOMATO~\cite{humantomato} introduces the first text-aligned whole-body motion generation that can generate high-quality, diverse, and coherent facial expressions, hand gestures, and body motions simultaneously.

\section{Limitation and Broader Impact}
\subsection{Limitation} There are two main limitations. \textbf{(i)} The motion quality of our markless motion annotation pipeline is inevitably inferior to the multi-view mark-based motion capture system. However, as the quantitative and qualitative results demonstrate, our method can perform much better than existing markless methods, thanks to large-scale models pre-trained on massive 2D and 3D keypoints datasets and our elaborately designed fitting pipeline. Besides, a 30 mm PA-MPVPE error would be acceptable for the text-driven motion generation task since the target is to synthesize natural and realistic motions that are semantically consistent with the text input. Furthermore,
the experiment on the mesh recovery task has demonstrated that our dataset can also benefit the human reconstruction task, which requires a higher annotation quality.
Accordingly, a better motion annotation will be beneficial, and we will leave it as our future work.
\textbf{(ii)} During our experiment, we found that existing evaluation metrics are not always consistent with visual results. Besides, SMPL-X parameters may not be the best motion representation for expressive whole-body motion representation. Thus, there is a need for further research on the evaluation metric, motion representation, and model designs for the expressive motion generation task. We leave them as future work.

\subsection{Broader Impact}

Based on the scalable and automatic annotation way proposed in this work, although there are inevitable errors, large-scale data could be helpful. Meanwhile, this way can boost the direction of ``learning from noisy labels" for related tasks, such as text-driven whole-body motion generation. 
A large-scale 3D human motion dataset would have numerous applications and boost novel research topics in various fields, such as animation, games, virtual reality, and human-computer interaction. Until now, human motion datasets have had no negative social impact. Our proposed \dataname will strictly follow the license of previous datasets, and would not present any negative foreseeable societal consequence, either.

\section{License}
All data is distributed under the CC BY-NC-SA (Attribution-NonCommercial-ShareAlike) license. Detailed license and instructions can be found on the page \url{https://motion-x-dataset.github.io}.  Further, we will provide a GitHub repository to solicit possible annotation errors from data users.
For the sub-datasets, we would ask the user to read the original license of each original dataset, and we would only provide our annotated result to the user with the approvals from the original Institution. Here, we provide a brief license of the used assets:

\begin{itemize}
    \item HumanML3D dataset~\cite{humanml3d} originates from the HumanAct12~\cite{guo2020action2motion} and AMASS~\cite{amass} datasets, which are both released for academic research only and it is free to researchers from educational or research institutes for non-commercial purposes. 
    \item BAUM dataset~\cite{baum} is CC-BY 4.0 licensed.
    \item HAA500 dataset~\cite{chung2021haa500} is MIT licensed. 
    \item IDEA400 dataset belongs to the International Digital Economy Academy (IDEA) and is licensed under the Attribution-Non Commercial-Share Alike 4.0 International License (CC-BY-NC-SA 4.0).
    \item UBC fashion dataset~\cite{UBCdwnet} is under the Creative Commons Attribution-NonCommercial 4.0 International (CC BY-NC 4.0) Public License.
    \item HuMMan dataset~\cite{cai2022humman}  is under S-Lab License v1.0.
    \item AIST dataset~\cite{li2021aist} is CC-BY 4.0 licensed.
    \item GRAB dataset~\cite{taheri2020grab} is released for academic research only and is free to researchers from educational or research institutes for non-commercial purposes.
    \item EgoBody~\cite{zhang2022egobody} is under CC-BY-NC-SA 4.0 license. 
    \item Other data is under CC BY-SA 4.0 license.
    \item SMPLify-X~\cite{smpl-x} codes are released for academic research only and are free to researchers from educational or research institutes for non-commercial purposes.
    \item Codes for preprocessing and training are under MIT LICENSE.

\end{itemize}
